# Supplementary material for: Improved return level estimation via a weighted likelihood, latent spatial extremes model
Source: arXiv:1810.07318 source file (2018-12-21)
Supplement: Supplementary file 1 [file weighted_spatial_gev_supplement.pdf]

# Supplement to "Improved return level estimation via a weighted likelihood latent spatial extremes model"

Joshua Hewitt, Miranda J. Fix, Jennifer A. Hoeting and Daniel S. Cooley

Colorado State University

## A Weights for completely dependent random variables

### A.1 Motivation for range of weights

We discuss the two special, limiting cases mentioned in Section 2.2 in more detail. If the field $\{Y_i(\boldsymbol{s})\}_{\boldsymbol{s}\in\mathcal{D}}$ has complete dependence over space, or is spatially independent, then the likelihood weights (5) yield the same statistical information about GEV parameters $\boldsymbol{\eta}$ as non-misspecified likelihoods, which fully account for extremal dependence. We justify this claim by showing that our weighted likelihood (4) is equivalent to non-misspecified likelihoods (A.1) in these special, limiting cases. We also make an informal argument that our weighted likelihood will approximate non-misspecified likelihoods in neighborhoods of these limiting cases.

Let $\boldsymbol{\gamma} \in \mathbb{R}^p$ be used generically to parameterize extremal dependence in the field $\{Y_i(\boldsymbol{s})\}_{\boldsymbol{s}\in\mathcal{D}}$ at time block $i \in \mathcal{T}$. Similarly, let the non-misspecified likelihood for observations $\{y_i(\boldsymbol{s}_j) : i \in \mathcal{T}, \boldsymbol{s}_j \in \mathcal{S}\}$ be defined via

$$L(\boldsymbol{\eta},\boldsymbol{\gamma}) = \prod_{i=1}^{T} f(y_i(\boldsymbol{s}_1),\dots,y_i(\boldsymbol{s}_N)|\,\boldsymbol{\eta},\boldsymbol{\gamma}). \tag{A.1}$$

Assume the joint density $f(y_i(\boldsymbol{s}_1),\dots,y_i(\boldsymbol{s}_N)|\,\boldsymbol{\eta},\boldsymbol{\gamma})$ is continuous with respect to $\boldsymbol{\gamma}$, and let the limiting conditions $\|\boldsymbol{\gamma}\| \to 0$ and $\|\boldsymbol{\gamma}\| \to \infty$ respectively parameterize fields that have no extremal dependence, and complete extremal dependence across space.

Alternative to the likelihood weights (5) we propose using, likelihood pseudo-weights $\{\tilde{w}_{\boldsymbol{s}_j,\boldsymbol{\gamma}} : j = 1, \ldots, N\}$ can be explicitly constructed to allow the non-misspecified likelihood (A.1) to be written in a weighted marginal form, such as

$$\prod_{i=1}^{T} f(y_i(\boldsymbol{s}_1), \ldots, y_i(\boldsymbol{s}_N) |\, \boldsymbol{\eta}, \boldsymbol{\gamma}) = \prod_{j=1}^{N}\prod_{i=1}^{T} f(y_i(\boldsymbol{s}_j) |\, \boldsymbol{\eta}(\boldsymbol{s}_j))^{\tilde{w}_{\boldsymbol{s}_j,\boldsymbol{\gamma}}}. \tag{A.2}$$

The pseudo-weights we will construct are purely theoretical tools because they cannot be computed in practice. Using pseudo-weights to express the non-misspecified likelihood (A.1) as a weighted marginal likelihood (A.2) implies the weighted likelihood we propose (4) will yield the same inference as non-misspecified likelihoods when our likelihood weights (5) are equivalent to the pseudo-weights. We refer to the alternative weights $\{\tilde{w}_{\boldsymbol{s}_j,\boldsymbol{\gamma}} : j = 1, \ldots, N\}$ as pseudo-weights because we will define them in (A.5) to depend on the joint density $f(y_i(\boldsymbol{s}_1), \ldots, y_i(\boldsymbol{s}_N) |\, \boldsymbol{\eta}, \boldsymbol{\gamma})$, which is not computationally tractable for spatially-referenced extremes data with $N > 10$, for example (Davison, Padoan, & Ribatet, 2012). Furthermore, computable pseudo-weights imply the joint density is available, thus the non-misspecified likelihood (A.1) may be used directly for inference and weighted likelihoods are unnecessary.

The likelihood pseudo-weights in (A.2) can be constructed in two parts. Begin by defining temporally-indexed weights $\{\tilde{w}_{i,\boldsymbol{\gamma}} : i = 1, \ldots, T\}$ that solve

$$f(y_i(\boldsymbol{s}_1), \ldots, y_i(\boldsymbol{s}_N) |\, \boldsymbol{\eta}, \boldsymbol{\gamma}) = \prod_{j=1}^{N} f(y_i(\boldsymbol{s}_j) |\, \boldsymbol{\eta}(\boldsymbol{s}_j))^{\tilde{w}_{i,\boldsymbol{\gamma}}}$$

for each $i \in \mathcal{T}$ via

$$\tilde{w}_{i,\boldsymbol{\gamma}} = \frac{\ln f(y_i(\boldsymbol{s}_1), \ldots, y_i(\boldsymbol{s}_N) |\, \boldsymbol{\eta}, \boldsymbol{\gamma})}{\sum_{j=1}^{N} \ln f(y_i(\boldsymbol{s}_j) |\, \boldsymbol{\eta}(\boldsymbol{s}_j))}. \tag{A.3}$$

That is, $\tilde{w}_{i,\boldsymbol{\gamma}}$ is the ratio of the log-likelihood contribution in (A.1) at time $i$ to the log-likelihood contribution from marginal likelihoods, which assume conditional independence.

The temporally-indexed weights (A.3) allow the likelihood (A.1) to be rewritten as

$$L(\boldsymbol{\eta}, \boldsymbol{\gamma}) = \prod_{j=1}^{N} \prod_{i=1}^{T} f(y_i(\boldsymbol{s}_j) | \, \boldsymbol{\eta}(\boldsymbol{s}_j))^{\tilde{w}_{i,\boldsymbol{\gamma}}}. \tag{A.4}$$

The desired likelihood weights $\left\{\tilde{w}_{\boldsymbol{s}_j,\boldsymbol{\gamma}} : j = 1, \ldots, N\right\}$, which are spatially-indexed, allow substitution of the inner product in (A.4) over $i = 1, \ldots, T$ by solving

$$\prod_{i=1}^{T} f(y_i(\boldsymbol{s}_j) | \, \boldsymbol{\eta}(\boldsymbol{s}_j))^{\tilde{w}_{\boldsymbol{s}_j,\boldsymbol{\gamma}}} = \prod_{i=1}^{T} f(y_i(\boldsymbol{s}_j) | \, \boldsymbol{\eta}(\boldsymbol{s}_j))^{\tilde{w}_{i,\boldsymbol{\gamma}}}$$

for each $\boldsymbol{s}_j \in \mathcal{S}$ via

$$\tilde{w}_{\boldsymbol{s}_j,\boldsymbol{\gamma}} = \frac{\sum_{i=1}^{T} \tilde{w}_{i,\boldsymbol{\gamma}} \ln f(y_i(\boldsymbol{s}_j) | \, \boldsymbol{\eta}(\boldsymbol{s}_j))}{\sum_{i=1}^{T} \ln f(y_i(\boldsymbol{s}_j) | \, \boldsymbol{\eta}(\boldsymbol{s}_j))}. \tag{A.5}$$

The likelihood weights we propose (5) converge to the pseudo-weights (A.5) as the extremal dependence approaches the special, limiting cases we consider. The extremal coefficient (1), combined with continuity of the joint density $f(y_i(\boldsymbol{s}_1), \ldots, y_i(\boldsymbol{s}_N) | \, \boldsymbol{\eta}, \boldsymbol{\gamma})$ with respect to $\boldsymbol{\gamma}$ imply our likelihood weights (5) satisfy $w_{\boldsymbol{s}_j} \to 1$ and $w_{\boldsymbol{s}_j} \to 1/N$, respectively as $\|\boldsymbol{\gamma}\| \to 0$ and $\|\boldsymbol{\gamma}\| \to \infty$. The pseudo-weights satisfy the same properties. In the first special case, convergence $\tilde{w}_{\boldsymbol{s}_j,\boldsymbol{\gamma}} \to 1$ as $\|\boldsymbol{\gamma}\| \to 0$ is immediate because the joint density converges to a product of independent densities $f(y_i(\boldsymbol{s}_1), \ldots, y_i(\boldsymbol{s}_N) | \, \boldsymbol{\eta}, \boldsymbol{\gamma}) \to \prod_{j=1}^{N} f(y_i(\boldsymbol{s}_j) | \, \boldsymbol{\eta}(\boldsymbol{s}_j))$. In the second special case, $\|\boldsymbol{\gamma}\| \to \infty$, convergence $\tilde{w}_{\boldsymbol{s}_j,\boldsymbol{\gamma}} \to 1/N$ can be seen since the limiting joint density factors as

$$\begin{aligned} f(y_i(\boldsymbol{s}_1), \ldots, y_i(\boldsymbol{s}_N) | \, \boldsymbol{\eta}) = & \prod_{j=1}^{N} f(y_i(\boldsymbol{s}_j) | \, \boldsymbol{\eta}(\boldsymbol{s}_j))^{1/N} \times \\ & \mathbb{1}\left\{F(y_i(\boldsymbol{s}_1) | \, \boldsymbol{\eta}(\boldsymbol{s}_1)) = \cdots = F(y_i(\boldsymbol{s}_N) | \, \boldsymbol{\eta}(\boldsymbol{s}_N))\right\} \end{aligned}$$

for certain configurations of marginal density parameters, such as when the data have common marginals. This is a result of Corollary A.1.1, presented and proved in Section A.2.

Convergence of the likelihood weights we propose (5) to the pseudo-weights (A.5) implies that the weighted likelihood we propose (4) also converges to the non-misspecified likelihood (A.1). Furthermore, convergence of the likelihoods allows us to informally claim that inference based on the two different likelihoods will be similar when data is sampled from a process with extremal dependence $\boldsymbol{\gamma}$ in a neighborhood of the limiting cases $\|\boldsymbol{\gamma}\| \to 0$ and $\|\boldsymbol{\gamma}\| \to \infty$.

## A.2 Theoretical results

Likelihood weights (A.3) and (A.5) are defined with respect to joint density functions. Completely dependent random variables have been studied in detail in the insurance industry, where they are referred to as comonotonic random variables. However, their joint density is not usually considered. Comonotonic random variables serve as basic models of worst-case scenarios for insurance portfolios, which makes the sum of comonotonic random variables more important than their joint distribution (Dhaene, Denuit, Goovaerts, Kaas, & Vyncke, 2002). To compute likelihood weights for completely dependent, or comonotonic variables, we first derive their joint density in Theorem A.1. Proofs for all results are presented in Section A.3.

**Theorem A.1.** *For any $j \in \{1, \dots, N\}$, the joint density $g(x_1, \dots, x_N)$ for a vector of comonotonic random variables $(X_1, \dots, X_N)$ can be parameterized as*

$$g(x_1, \dots, x_N) = f_j(x_j)\mathbb{1}(F_1(x_1) = \cdots = F_N(x_N)) \tag{A.6}$$

*where $F_j$ and $f_j$ respectively denote the cumulative distribution function and density for $X_j$ relative to Lebesgue measure on $\mathbb{R}$. The density (A.6) is defined with respect to the dominating measure $\lambda_N + \lambda_{\mathcal{C}}$ for which $\lambda_N$ is Lebesgue measure on $\mathbb{R}^N$ and $\lambda_{\mathcal{C}}$ is Lebesgue measure on $\mathcal{C} = \{(x_1, \dots, x_N) : F_1(x_1) = \cdots = F_N(x_N)\} \subset \mathbb{R}^N$.*

While Theorem A.1 allows the likelihood weights (A.3) and (A.5) to be computed, devel-

oping intuition requires additional theory because the density (A.6) only explicitly includes one density $f_j$. Lemma A.1 will allow the likelihood weights to be manipulated by providing a means to express $f_i$ as a rescaling of $f_j$ for $i \neq j$.

**Lemma A.1.** *For a vector of comonotonic random variables $(X_1, \ldots, X_N)$, the marginal density $f_i(x_i)$ for $X_i$ may be re-expressed in terms of $f_j(x_j)$ using function composition $\circ$ and the quantile density function $q(u) = \frac{\partial}{\partial u} F^{-1}(u)$ through*

$$f_i(x_i) = f_j(x_j) \frac{(q_j \circ F_j)(x_j)}{(q_i \circ F_j)(x_j)} \tag{A.7}$$

*for any $j = 1, \ldots, N$, continuous $F_i, F_j$, and $x_j$ s.t. $F_i(x_i) = F_j(x_j)$.*

Intuition for the likelihood weights (A.3) and (A.5) follows from algebraic manipulation. In particular, Corollary A.1.1 yields conditions under which likelihood weights are intuitive (e.g., $w_{(j)} = N^{-1}$), such as when $X_1, \ldots, X_N$ have common marginals.

**Corollary A.1.1.** *For any $j \in \{1, \ldots, N\}$, the likelihood weight (A.3) for a single vector of comonotonic random variables $(X_1, \ldots, X_N)$ is*

$$w_{(j)} = \frac{1}{N + d_{(j)}} \tag{A.8}$$

*where*

$$d_{(j)} = \frac{1}{\ln f_j(x_j)} \sum_{i=1}^{N} \ln \frac{(q_j \circ F_j)(x_j)}{(q_i \circ F_j)(x_j)}$$

*and the subscript highlights the dependence of the weight $w_{(j)}$ on the density $f_j$ used to parameterize the comonotonic density $g$. The average weight across all parameterizations is*

$$\bar{w} = \frac{1}{N} \sum_{j=1}^{N} w_{(j)} = \frac{1}{N}.$$

## A.3 Proofs of theoretical results

### A.3.1 Completely dependent densities: Proof of Theorem A.1

A random vector of comonotonic variables $(X_1, \dots, X_N)$ has support $\mathcal{C}$ and cumulative distribution function (CDF) given by

$$F(x_1, \dots, x_N) = \min_{i \in \{1,\dots,N\}} F_i(x_i)$$

where $F_i$ is the CDF for $X_i$ (Dhaene et al., 2002, Theorem 2). The CDF $F$ and support $\mathcal{C}$ imply the probability measure $\mathcal{P}$ associated with $F$ is absolutely continuous with respect to $\lambda_N + \lambda_{\mathcal{C}}$. Integrating (A.6) over a half-infinite rectangle
$A = \{(y_1, \dots, y_N) : y_i \leq x_i, i = 1, \dots, N\}$ yields $F(x_1, \dots, x_N)$ since

$$\text{(A.9)} \qquad \int_A g(y_1, \dots, y_N) d(\lambda_N + \lambda_{\mathcal{C}}) = \int_{-\infty}^{F_j^{-1}(\min_i F_i(x_i))} f_j(y) dy$$

$$\text{(A.10)} \qquad = P\Big(U \leq \min_i F_i(x_i)\Big), \; U \sim U(0,1)$$

$$\text{(A.11)} \qquad = \min_{i \in \{1,\dots,N\}} F_i(x_i).$$

The integral (A.9) simplifies because $g$ is measure-0 with respect to $\lambda_N$ and a 1:1 mapping exists between $A \cap \mathcal{C}$ and $\mathbb{R}$ since for any $j \in \{1, \dots, N\}$

$$\begin{aligned} A \cap \mathcal{C} &= \{(y_1, \dots, y_N) : F_1(y_1) = \cdots = F_N(y_N); \; F_i(y_i) \leq F_i(x_i), i = 1, \dots, N\} \\ &= \Big\{(y_1, \dots, y_N) : F_1(y_1) = \cdots = F_N(y_N); \; F_j(y_j) \leq \min_i F_i(x_i)\Big\} \\ &= \Big\{(y_1, \dots, y_N) : F_1(y_1) = \cdots = F_N(y_N); \; y_j \leq F_j^{-1}\Big(\min_i F_i(x_i)\Big)\Big\}. \end{aligned}$$

The probability integral transformation yields (A.10), from which (A.11) naturally follows. The Radon-Nikodym theorem and general properties of distribution functions imply $g$ is a density for $(X_1, \dots, X_N)$ with respect to $\lambda_N + \lambda_{\mathcal{C}}$.

### A.3.2 Rescaled marginal densities: Proof of Lemma A.1

The rescaling (A.7) uses the identity

$$(f \circ Q)(u)q(u) = 1, u \in [0, 1] \tag{A.12}$$

in which $Q(u) = F^{-1}(u)$ is the quantile function for a continuous cumulative distribution function $F$ (Parzen, 1979, eqn. 2.6). The support constraint $F_i(x_i) = F_j(x_j)$ implies $x_i = (Q_i \circ F_j)(x_j)$ and allows $f_i(x_i)$ to be rewritten as

$$f_i(x_i) = (f_i \circ Q_i \circ F_j)(x_j). \tag{A.13}$$

The desired result (A.7) follows from applying the identity (A.12) twice to (A.13) since

$$\begin{aligned} f_i(x_i) =& \{(q_i \circ F_j)(x_j)\}^{-1} \\ =& \frac{(f_j \circ Q_j \circ F_j)(x_j)(q_j \circ F_j)(x_j)}{(q_i \circ F_j)(x_j)} \\ =& f_j(x_j)\frac{(q_j \circ F_j)(x_j)}{(q_i \circ F_j)(x_j)}. \end{aligned}$$

### A.3.3 Completely dependent weights: Proof of Corollary A.1.1

Theorem A.1 implies the likelihood weight (A.3) for a single vector of comonotonic random variables $(X_1, \ldots, X_N)$ is

$$w_{(j)} = \frac{\ln f_j(x_j)}{\sum_{i=1}^N \ln f_i(x_i)} \tag{A.14}$$

for all $(x_1, \ldots, x_N)$ that satisfy the support constraint $F_1(x_1) = \cdots = F_N(x_N)$. Lemma A.1 yields the first result (A.8) as it lets us re-express the denominator of (A.14) in terms of

$f_j(x_j)$ as

$$\sum_{i=1}^{N} \ln f_i(x_i) = \sum_{i=1}^{N} \left( \ln f_j(x_j) + \ln \frac{(q_j \circ F_j)(x_j)}{(q_i \circ F_1)(x_j)} \right)$$
$$= \ln f_j(x_j) \big( N + d_{(j)} \big)$$

where

$$d_{(j)} = \frac{1}{\ln f_j(x_j)} \sum_{i=1}^{N} \ln \frac{(q_j \circ F_j)(x_j)}{(q_i \circ F_j)(x_j)}.$$

The average weight $\bar{w}$ follows directly from (A.14) since

$$\bar{w} = \frac{1}{N} \sum_{j=1}^{N} \frac{\ln f_j(x_j)}{\sum_{i=1}^{N} \ln f_i(x_i)} = \frac{1}{N}.$$

# B Bayesian implementation of model

We describe a Gibbs sampler that draws samples from the posterior distribution of latent spatial extremes models that use weighted or penalized likelihoods, respectively (4) or (8) (Section B.1). We also describe our choice of prior distributions and the parameterizations we use in our simulation study (Section B.2.1) and application to Colorado precipitation (Section B.2.2).

## B.1 Gibbs sampler

Gibbs sampling begins by updating marginal GEV parameters at the sampling locations $\{\boldsymbol{\eta}(\boldsymbol{s}_j) : j = 1, \ldots, N\}$. The parameter vectors are updated sequentially, from $j = 1, \ldots, N$. Separate random walk Metropolis-Hastings steps—respectively with fixed proposal standard deviations $s_\mu$, $s_{\log\sigma}$, and $s_\xi$—are used to update the entries of each parameter vector $\boldsymbol{\eta}(\boldsymbol{s}_j) = (\mu(\boldsymbol{s}_j), \log\sigma(\boldsymbol{s}_j), \xi(\boldsymbol{s}_j))^T$. Proposal standard deviations are chosen in preliminary test runs of the Gibbs sampler to tune acceptance rates so they are close to 44% (Roberts

& Rosenthal, 2001).

Sampling then proceeds to update regression coefficients $\boldsymbol{\beta}$ and spatial covariance parameters $\boldsymbol{\phi} = (\sigma_0, \lambda_0, \nu_0)^T$ for each of the independent Gaussian process priors for the GEV parameter processes $\{\mu(\boldsymbol{s})\}_{\boldsymbol{s}\in\mathcal{D}}$, $\{\log\sigma(\boldsymbol{s})\}_{\boldsymbol{s}\in\mathcal{D}}$, and $\{\xi(\boldsymbol{s})\}_{\boldsymbol{s}\in\mathcal{D}}$. Regression coefficients and spatial covariance parameters determine the mean and covariance structures of the Gaussian processes. Separate random walk Metropolis-Hastings steps update spatial range $\lambda_0$ and smoothness $\nu_0$ parameters. The random walk proposal distributions respectively have fixed proposal standard deviations $s_{\lambda_0}$ and $s_{\nu_0}$, which are specified for each of the Gaussian processes. Regression coefficients $\boldsymbol{\beta}$ and sills $\sigma_0$ are sampled from conjugate distributions.

For example, the Gaussian process assumption in Section 2.4 implies the collection of GEV location parameters $\boldsymbol{\mu} = [\mu(\boldsymbol{s}_j)]_{j=1}^N \in \mathbb{R}^N$ have the conditional prior distribution $\boldsymbol{\mu}|\,\boldsymbol{\beta}_\mu, \boldsymbol{\phi}_\mu \sim \mathcal{N}\big(X_\mu\boldsymbol{\beta}_\mu, \Sigma_\mu\big)$, where the matrix $X_\mu \in \mathbb{R}^{N\times p_\mu}$ is composed of the $N$ row vectors $\boldsymbol{x}_\mu(\boldsymbol{s}_j)^T \in \mathbb{R}^{p_\mu}$, $j = 1,\ldots,N$, and $\Sigma_\mu \in \mathbb{R}^{N\times N}$ is a spatial covariance matrix with entries $(\Sigma_\mu)_{ij} = \rho\big(\|\boldsymbol{s}_i - \boldsymbol{s}_j\|\,;\boldsymbol{\phi}_\mu\big)$. Since the regression coefficients have prior distribution $\boldsymbol{\beta}_\mu \sim \mathcal{N}(\boldsymbol{0}, \Lambda_\mu)$ in which $\Lambda_\mu$ is a fixed prior covariance matrix, the conjugate full conditional posterior distribution for $\boldsymbol{\beta}_\mu$ is $\boldsymbol{\beta}_\mu\big|\,\boldsymbol{\mu}, \boldsymbol{\phi}_\mu, \cdot \sim \mathcal{N}(m, \Psi)$ with covariance $\Psi = \big(\Lambda_\mu^{-1} + X_\mu^T\Sigma_\mu X_\mu\big)^{-1}$ and mean $m = \Psi X_\mu^T\Sigma_\mu^{-1}\boldsymbol{\mu}$. The covariance sill has inverse gamma prior distribution $\sigma_0 \sim \mathrm{IG}\,(a_\mu, b_\mu)$ and conjugate full conditional posterior distribution that depends on the current iteration of the Gaussian process parameters and values $\sigma_0|\,\boldsymbol{\mu}, \boldsymbol{\beta}_\mu, \lambda_\mu, \nu_\mu, \cdot \sim \mathrm{IG}\,\big(a_\mu + N/2, b_\mu + e^T(\Sigma_\mu/\sigma_0)^{-1}e/2\big)$ where $e = \boldsymbol{\mu} - X_\mu\boldsymbol{\beta}_\mu$. The conjugate distributions for the regression and sill parameters of the other Gaussian processes $\{\log\sigma(\boldsymbol{s})\}_{\boldsymbol{s}\in\mathcal{D}}$ and $\{\xi(\boldsymbol{s})\}_{\boldsymbol{s}\in\mathcal{D}}$ use similar notation and results for their Gibbs steps.

If the model is being fit with Gibbs-updated likelihood weights or penalties, the weights and penalty tuning parameters are updated next. Likelihood weights are computed from (5), in which a plug-in estimator $\hat{\theta}(d)$ is used for the extremal coefficient. The plug-in estimator $\hat{\theta}(d)$ is only a function of the data and marginal parameters, so does not explicitly rely on the dependence parameter $\gamma$. The basis for the plug-in estimator is a relation-

ship between the extremal coefficient and the F-madogram $\nu^F(d)$. The F-madogram is an analog of the classical variogram for spatial statistics and measures spatial dependence in stationary max-stable fields. If the marginal GEV shape parameters satisfy $\xi(\boldsymbol{s}) < 1$ (i.e., they are not too large), then the extremal coefficient is related to the F-madogram via $\theta(d) = \big(1 + 2\nu^F(d)\big)/\big(1 - 2\nu^F(d)\big)$ (Cooley, Naveau, & Poncet, 2006). After using marginal parameters $\boldsymbol{\eta}$ to transform data $\{y_i(\boldsymbol{s}_j) : i \in \mathcal{T}, j \in \mathcal{S}\}$ to have unit Fréchet margins, the sample F-madogram can be estimated in a similar manner as variograms, by working with the differences between pairs of observations separated by a distance $d$. Likelihood weights may be estimated before Gibbs sampling by using the empirical cumulative distribution function (CDF) to transform the data to have unit Fréchet margins in order to estimate the sample F-madogram. Uncertainty in the likelihood weights (5) can also be incorporated by updating them at each Gibbs iteration. Conditional on the data and marginal parameters, the weights are deterministic because the sample F-madogram is deterministic. Thus, the weights do not need to be sampled; weights can be updated by using the marginal parameters $\boldsymbol{\eta}$ to re-transform the data to re-estimate the F-madogram at each Gibbs iteration.

The plug-in estimator $\hat{\theta}(d)$ is updated by using the current Gibbs values of the GEV parameters at the sampling locations $\{\boldsymbol{\eta}(\boldsymbol{s})\}_{\boldsymbol{s}\in\mathcal{S}}$ to transform the data $\{y_i(\boldsymbol{s}_j) : i \in \mathcal{T}, j \in \mathcal{S}\}$ to have unit Fréchet margins. The plug-in estimator $\hat{\theta}(d)$ is recomputed from an estimate of the sample F-madogram, using the transformed data. If the model is using a penalized likelihood, as in Section 3.2.1 and (8), the penalty's tuning parameter $\lambda$ may be updated as well. The penalized complexity prior (C.1) does not have a conjugate distribution, so must be updated with a random walk Metropolis-Hastings step. Unlike the other random walk updates, the sampler uses a basic version of Algorithm 4 from Andrieu and Thoms (2008) to adaptively tune the proposal standard deviation $s_\lambda$ during estimation so the acceptance rate is close to 44%.

Table 1: Prior distributions used in simulation study (Section 3.2).

| | GEV parameter process | | |
|---|---|---|---|
| | $\{\mu(\boldsymbol{s})\}_{\boldsymbol{s}\in\mathcal{D}}$ | $\{\log\sigma(\boldsymbol{s})\}_{\boldsymbol{s}\in\mathcal{D}}$ | $\{\xi(\boldsymbol{s})\}_{\boldsymbol{s}\in\mathcal{D}}$ |
| *(Regression coefs.)* | | | |
| $\boldsymbol{\beta}\sim$ | $\mathcal{N}\left(\mathbf{0}, \begin{bmatrix} 400 & \\ & 100 \end{bmatrix}\right)$, | $\mathcal{N}\left(\mathbf{0}, \begin{bmatrix} 400 & \\ & 100 \end{bmatrix}\right)$, | $\mathcal{N}(0, 100)$. |
| *(Spatial covariance)* | | | |
| $\sigma_0 \sim$ | $\text{IG}(1, 8)$, | $\text{IG}(1, .8)$, | $\text{IG}(1, .0024)$. |
| $\lambda_0 \sim$ | $\text{Gamma}(2, 10)$, | $\text{Gamma}(2, 2.5)$, | $\text{Gamma}(2, 5)$. |

## B.2 Specification of prior distributions

### B.2.1 Simulation

Prior distributions for regression coefficients $\boldsymbol{\beta}$ and spatial covariance parameters $\sigma_0$ and $\lambda_0$ used in the simulation study (Section 3) are specified in Table 1. The spatial smoothness $\nu_0$ is fixed at the truth. Regression coefficient prior distributions are designed to be uninformative, while the spatial covariance prior distributions are designed to be weakly informative. The spatial covariance prior distributions have infinite or large variation. The distributions are parameterized such that the mean of the priors are centered at the true generating model parameters for the spatial range $\lambda_0$; the mode of the priors for the sill parameters $\sigma_0$ are centered at the true generating model parameters. The penalized complexity prior parameter has prior distribution $\lambda \sim \text{IG}(2, 1)$. The proposal standard deviations for the random walk Metropolis-Hastings samplers are $s_\mu = 1.2$, $s_{\log\sigma} = .08$, $s_\xi = .08$; and $s_{\lambda_0}$ is .7, .8. and .7, respectively for the GEV location $\{\mu(\boldsymbol{s})\}_{\boldsymbol{s}\in\mathcal{D}}$, scale $\{\log\sigma(\boldsymbol{s})\}_{\boldsymbol{s}\in\mathcal{D}}$, and shape $\{\xi(\boldsymbol{s})\}_{\boldsymbol{s}\in\mathcal{D}}$ processes.

Table 2: Prior distributions used in application to extreme Colorado precipitation (Section 4).

| | GEV parameter process | | |
|---|---|---|---|
| | $\{\mu(\boldsymbol{s})\}_{\boldsymbol{s}\in\mathcal{D}}$ | $\{\log\sigma(\boldsymbol{s})\}_{\boldsymbol{s}\in\mathcal{D}}$ | $\{\xi(\boldsymbol{s})\}_{\boldsymbol{s}\in\mathcal{D}}$ |
| *(Regression coefs.)* | | | |
| $\boldsymbol{\beta} \sim$ | $\mathcal{N}(0, 100)$, | $\mathcal{N}(0, 100)$, | $\mathcal{N}(0, 100)$. |
| *(Spatial covariance)* | | | |
| $\sigma_0 \sim$ | $\text{IG}\,(2, 60)$, | $\text{IG}\,(2, 10)$, | $\text{IG}\,(2, .03)$. |
| $\lambda_0 \sim$ | $\text{Gamma}\,(2, .5)$, | $\text{Gamma}\,(2, .25)$, | $\text{Gamma}\,(2, .1)$. |
| $\nu_0 \sim$ | $\text{Gamma}\,(2, 1)$, | $\text{Gamma}\,(2, 1)$, | $\text{Gamma}\,(2, 1)$. |

#### B.2.2 Colorado application

Prior distributions for regression coefficients $\boldsymbol{\beta}$ and spatial covariance parameters $\sigma_0$ and $\lambda_0$ used in the application to extreme Colorado precipitation (Section 4) are specified in Table 1. Regression coefficient prior distributions are designed to be uninformative, while the spatial covariance prior distributions are designed to be weakly informative. The spatial covariance prior large variance. The distributions are parameterized such that the prior mode covers least-square variogram estimates for the spatial covariance parameters. Variograms are based on smoothed maximum likelihood fits of the GEV parameters. The proposal standard deviations for the random walk Metropolis-Hastings samplers are $s_\mu = 1.45$, $s_{\log\sigma} = .25$, $s_\xi = .11$; $s_{\lambda_0}$ is .3, .4. and .6, respectively for the GEV location $\{\mu(\boldsymbol{s})\}_{\boldsymbol{s}\in\mathcal{D}}$, scale $\{\log\sigma(\boldsymbol{s})\}_{\boldsymbol{s}\in\mathcal{D}}$, and shape $\{\xi(\boldsymbol{s})\}_{\boldsymbol{s}\in\mathcal{D}}$ processes; similarly, $s_{\nu_0}$ is .12, .1, and .15.

### B.3 Posterior diagnostics for Colorado application

Posterior diagnostics do not suggest the Gibbs sampler has not converged. Similarly, posterior diagnostics suggest the sampler has been run for a long enough period of time and is able to identify model parameters from the data. In particular, there is no strong evidence that posterior inference is sensitive to the sampler's initial state. We use potential scale reduction

factors (PSRFs) to assess posterior convergence by comparing inference from nine independent copies of our Gibbs sampler. Potential scale reduction factors estimate the potential reduction in uncertainty of posterior means if the Gibbs samplers were allowed to run for an infinitely longer amount of time (Gelman & Rubin, 1992). Each copy of the sampler was randomly initialized by drawing model parameters from the model's prior distribution. The maximum upper confidence limit of PSRFs for return levels at the observation locations is 1.04, suggesting that the posterior uncertainty in return levels is inflated by up to 4% due to Gibbs sampling. A multivariate extension of the PSRFs estimates the largest potential scale reduction factor among all linear combinations of a collection of posterior means (Brooks & Gelman, 1998). For return levels, this quantity is also 1.04. The multivariate PSRFs for GEV location and scale parameters are each 1.01, and the multivariate PSRF for GEV shape parameters is 1.05.

Posterior traceplots, autocorrelation plots, and effective sample sizes indicate the Gibbs sampler is slowly mixing, but additional diagnostics suggest the sampler has been run for enough samples so as to control Monte Carlo integration error. Estimates of the Monte Carlo integration error are small relative to the magnitude of posterior means of interest, such as posterior means for marginal return levels, latent GEV parameters, and the spatial mean and covariance functions of the spatial processes that model the GEV parameters. In particular, Monte Carlo integration errors are at most .6% of the magnitude of posterior return levels, scale parameters, and location parameters. Monte Carlo integration errors are at most 3.4% the magnitude of posterior shape parameters. The relative sizes of Monte Carlo errors are more variable for the mean and covariance function parameters of the latent GEV parameter fields, but are between .1% and 2.5% for all mean and covariance function parameters except for three parameters. Monte Carlo integration errors are respectively 4.5% and 6.1% of the magnitude of the posterior mean for the smoothness parameters $\nu_0$ of the GEV scale $\{\sigma^2(\boldsymbol{s})\}_{\boldsymbol{s}\in\mathcal{D}}$ and shape $\{\xi(\boldsymbol{s})\}_{\boldsymbol{s}\in\mathcal{D}}$ parameter processes. Lastly, Monte Carlo integration error is 37% of the magnitude of the posterior mean for the effect of mean annual

precipitation $\beta_1$ on shape parameters $\{\xi(\boldsymbol{s})\}_{\boldsymbol{s}\in\mathcal{D}}$. However, this ratio is artificially inflated because the parameter is estimated to be small or vanishing ($\hat{\beta}_1 = .001$; 95% highest posterior density interval is $(-.04, .04)$ ).

Posterior diagnostics also suggest the data at least weakly identify the mean and covariance parameters for the latent GEV parameter fields. The posterior densities for the mean functions of the Gaussian processes used to model the GEV parameters all differ from the prior distributions (Figure 1, Figure 3, Figure 5). Similarly, posterior densities for the parameters of the spatial covariance functions for the latent GEV parameters differ from the prior densities (Figure 2, Figure 4, Figure 6). However, the posterior distributions do not differ dramatically from the priors for the smoothness and range parameters of the covariance function $\rho_{\xi(\boldsymbol{s})}$ of the GEV shape parameters.

# C Penalized complexity prior for the GEV shape parameter $\xi$

Following Simpson, Rue, Riebler, Martins, and Sørbye (2017), the penalized complexity prior for the generalized extreme value (GEV) distribution (2) is defined through the prior density

$$\pi(\xi|\,\lambda) = \lambda e^{-\lambda d(\xi)} \left|\frac{\partial d(\xi)}{\partial \xi}\right| \tag{C.1}$$

with tuning parameter $\lambda > 0$ and "distance" function $d(\xi) = \sqrt{2\,\mathrm{KLD}\,(f_\xi \| f_{\xi_0})}$. The distance function $d(\xi)$ is based on the Kullback-Leibler divergence $\mathrm{KLD}\,(f_\xi \| f_{\xi_0})$ between the GEV distribution with shape parameter $\xi$ and reference shape parameter $\xi_0$. The penalized complexity prior encourages shrinkage of the shape parameter $\xi$ toward the reference parameter $\xi_0$. A natural choice for the reference parameter is $\xi_0 = 0$, the point at which the GEV distribution changes from having a heavy tail ($\xi > 0$) to a light tail ($\xi < 0$). The

Kullback-Leibler divergence is

$$\begin{aligned}\mathrm{KLD}\left(f_\xi \| f_{\xi_0}\right) &= \int_{\mathbb{S}} f_\xi(y) \log \frac{f_\xi(y)}{f_{\xi_0}(y)} dy \\ &= \int_{\mathbb{S}} \frac{1}{\sigma} t_\xi(y)^{\xi+1} \exp\left\{-t_\xi(y)\right\} \log\left(\frac{t_\xi(y)^{\xi+1}\exp\left\{-t_\xi(y)\right\}}{e^{-(y-\mu)/\sigma}\exp\left\{-e^{-(y-\mu)/\sigma}\right\}}\right) dy \\ &= (\xi+1)\psi(1) - 1 + (\Gamma(1-\xi)-1)/\xi + \exp\left\{1/\xi\right\} \mathrm{I}_\xi\end{aligned} \tag{C.2}$$

where $t_\xi(y) = (1+\xi(y-\mu)/\sigma)^{-1/\xi}$, $\psi(\cdot)$ is the digamma function, $I_\xi = \int_0^\infty \exp\left\{-\left(\xi s^\xi\right)^{-1}\right\} e^{-s} ds$, and $\mathbb{S} = [\mu - \sigma/\xi, \infty)$ is the distribution's support for $\xi > 0$. When $\xi < 0$, the support is reversed $\mathbb{S} = (-\infty, \mu - \sigma/\xi]$. The definite integral $I_\xi$ does not simplify analytically but includes the $e^{-s}$ "weight function" so can be efficiently approximated numerically with Gauss-Laguerre quadrature (Givens & Hoeting, 2013, Section 5.3). The Kullback-Leibler divergence is trivially zero when $\xi = 0$ but otherwise expands to (C.2), the sum of the integrals (C.3) to (C.6). The first integral (C.3) uses the substitution $s = \log t_\xi(y)$, yielding

$$\begin{aligned}(\xi+1)\int_{\mathbb{S}} \frac{1}{\sigma} t_\xi(y)^{\xi+1} \exp\left\{-t_\xi(y)\right\} \log t_\xi(y) dy &= (\xi+1)\int_{\mathbb{R}} s \exp\left\{s - e^s\right\} ds \\ &= (\xi+1)\psi(1).\end{aligned} \tag{C.3}$$

The transformed integral in (C.3) represents $-1$ times the expected value for a standard Gumbel random variable, allowing simplification. The second integral (C.4) uses the substitution $s = t_\xi(y)$, yielding

$$-\int_{\mathbb{S}} \frac{1}{\sigma} t_\xi(y)^{\xi+1} \exp\left\{-t_\xi(y)\right\} t_\xi(y) dy = -\int_0^\infty s e^{-s} ds = -1. \tag{C.4}$$

For $\xi < 1$ and $\xi \neq 0$, the third integral (C.5) is exactly equivalent to

$$\mathrm{E}_\xi\left[(y-\mu)/\sigma\right] = (\Gamma(1-\xi)-1)/\xi. \tag{C.5}$$

The last integral (C.6) also uses the substitution $s = t_\xi(y)$, yielding

$$\int_{\mathbb{S}} \frac{1}{\sigma} t_\xi(y)^{\xi+1} \exp\{-t_\xi(y)\} \exp\{-(y-\mu)/\sigma\}\, dy = \exp\{1/\xi\}\, I_\xi. \tag{C.6}$$

The penalized complexity prior (C.1) also requires the distance function's derivative $\frac{\partial}{\partial\xi} d(\xi) = \left(2\,\mathrm{KLD}\left(f_\xi \| f_{\xi_0}\right)\right)^{-1/2} \frac{\partial}{\partial\xi} \mathrm{KLD}\left(f_\xi \| f_{\xi_0}\right)$. While differentiating the Kullback-Leibler divergence (C.2) is straightforward

$$\frac{\partial}{\partial\xi} \mathrm{KLD}\left(f_\xi \| f_{\xi_0}\right) = \psi(1) - \frac{\Gamma(1-\xi)(\xi\psi(1-\xi)+1)-1}{\xi^2} + \exp\{1/\xi\}\left(\frac{\partial}{\partial\xi} I_\xi - \frac{I_\xi}{\xi^2}\right),$$

evaluating the derivative also requires Gauss-Laguerre approximation of the definite integral

$$\frac{\partial}{\partial\xi} I_\xi = \int_0^\infty \frac{1+\xi\log s}{\xi^2 s^\xi} \exp\left\{-\left(\xi s^\xi\right)^{-1}\right\} e^{-s} ds.$$

# D Additional simulation results

Figure 8 through Figure 19 present empirical coverage, mean squared error, and relative bias for all GEV parameters $\mu(\boldsymbol{s})$, $\sigma(\boldsymbol{s})$, and $\xi(\boldsymbol{s})$ for all combinations of estimation models and generating model configurations used in the simulation study described in Section 3. Relative bias is the estimator bias scaled by the truth, for example

$$\text{Rel. Bias}(\mu(\boldsymbol{s})) = \frac{\mathrm{E}\left[\hat{\mu}(\boldsymbol{s}) - \mu(\boldsymbol{s})\right]}{\mu(\boldsymbol{s})} \times 100\%.$$

# E Additional Colorado results

The weighted likelihood model induces shrinkage of the GEV parameters $\boldsymbol{\eta}(\boldsymbol{s})$ and return levels $Q(p|\,\boldsymbol{\eta}(\boldsymbol{s}))$ (Figure 21). In hierarchical models, estimates balance data with smoothness constraints imposed by hierarchical layers. Shrinkage occurs in the weighted model because

the weighted model shifts the balance more toward the hierarchical layers.

# References

Andrieu, C., & Thoms, J. (2008). A tutorial on adaptive MCMC. *Statistics and Computing*, *18*, 343–373.

Brooks, S. P., & Gelman, A. (1998). General Methods for Monitoring Convergence of Iterative Simulations. *Journal of Computational and Graphical Statistics*, *7*(4), 434–455.

Cooley, D., Naveau, P., & Poncet, P. (2006). Variograms for spatial max-stable random fields. In P. Bertail, P. Doukhan, & P. Soulier (Eds.), *Dependence in probability and statistics* (pp. 373–390). New York, NY: Springer Science+Business Media, LLC.

Davison, A. C., Padoan, S. A., & Ribatet, M. (2012). Statistical Modeling of Spatial Extremes. *Statistical Science*, *27*(2), 161–186.

Dhaene, J., Denuit, M., Goovaerts, M. J., Kaas, R., & Vyncke, D. (2002). The concept of comonotonicity in actuarial science and finance : theory. *Insurance: Mathematics and Economics*, *31*, 3–33.

Gelman, A., & Rubin, D. B. (1992). Inference from Iterative Simulation Using Multiple Sequences. *Statistical Science*, *7*(4), 457–511.

Givens, G. H., & Hoeting, J. A. (2013). *Computational Statistics* (Second ed.). Hoboken, NJ: John Wiley & Sons, Inc.

Parzen, E. (1979). Nonparametric Statistical Data Modeling. *Journal of the American Statistical Association*, *74*(365), 105–121.

Roberts, G. O., & Rosenthal, J. S. (2001). Optimal scaling for various Metropolis-Hastings algorithms. *Statistical Science*, *16*(4), 351–367.

Simpson, D., Rue, H., Riebler, A., Martins, T. G., & Sørbye, S. H. (2017). Penalising Model Component Complexity : A Principled , Practical Approach to Constructing Priors.

*Statistical Science*, *32*(1), 1–28.

# List of Figures

1 Comparison of prior and posterior distributions for the mean function of the latent Gaussian process that models GEV location parameters $\{\mu(\boldsymbol{s})\}_{\boldsymbol{s}\in\mathcal{D}}$ . . 21
2 Comparison of prior and posterior distributions for the covariance parameters of the latent Gaussian process that models GEV location parameters $\{\mu(\boldsymbol{s})\}_{\boldsymbol{s}\in\mathcal{D}}$ 22
3 Comparison of prior and posterior distributions for the mean function of the latent Gaussian process that models GEV scale parameters $\{\sigma^2(\boldsymbol{s})\}_{\boldsymbol{s}\in\mathcal{D}}$ . . . 23
4 Comparison of prior and posterior distributions for the covariance parameters of the latent Gaussian process that models GEV scale parameters $\{\sigma^2(\boldsymbol{s})\}_{\boldsymbol{s}\in\mathcal{D}}$ 24
5 Comparison of prior and posterior distributions for the mean function of the latent Gaussian process that models GEV shape parameters $\{\xi(\boldsymbol{s})\}_{\boldsymbol{s}\in\mathcal{D}}$ . . . 25
6 Comparison of prior and posterior distributions for the covariance parameters of the latent Gaussian process that models GEV shape parameters $\{\xi(\boldsymbol{s})\}_{\boldsymbol{s}\in\mathcal{D}}$ 26
7 Empirical mean squared error (MSE) of posterior estimates for 100-year return levels $Q(.99|\,\boldsymbol{\eta}(\boldsymbol{s}))$ for four levels of extreme dependence across comparison models and simulations with $T = 50$ observations per location. The weighted model has similar or better performance than the standard, unweighted model in nearly all simulations. The unweighted model underestimates uncertainty, so has slightly smaller MSE for the simulation with strong extremal dependence. Supplement Section D includes results for $T = 100$, which show slight reduction in MSE. . . . . . . . . . . . . . . . . . . . . . . . . . . . . . . . 27
8 Empirical coverage rates of 95% highest posterior density intervals for 100-year return levels $Q(.99|\,\boldsymbol{\eta}(\boldsymbol{s}))$ across comparison models and all simulations. Nominal coverage is marked by the dotted horizontal reference line at .95. . . 28
9 Empirical coverage rates of 95% highest posterior density intervals for GEV location parameters $\mu(\boldsymbol{s})$ across comparison models and all simulations . . . 29
10 Empirical coverage rates of 95% highest posterior density intervals for GEV scale parameters $\sigma(\boldsymbol{s})$ across comparison models and all simulations . . . . . 30
11 Empirical coverage rates of 95% highest posterior density intervals for GEV shape parameters $\xi(\boldsymbol{s})$ across comparison models and all simulations . . . . . 31
12 Empirical mean square error (MSE) of posterior estimates for 100-year return levels $Q(.99|\,\boldsymbol{\eta}(\boldsymbol{s}))$ across comparison models and all simulations. . . . . . . . 32
13 Empirical mean square error (MSE) of posterior estimates for GEV location parameters $\mu(\boldsymbol{s})$ across comparison models and all simulations . . . . . . . . 33
14 Empirical mean square error (MSE) of posterior estimates for GEV scale parameters $\sigma(\boldsymbol{s})$ across comparison models and all simulations . . . . . . . . 34
15 Empirical mean square error (MSE) of posterior estimates for GEV shape parameters $\xi(\boldsymbol{s})$ across comparison models and all simulations . . . . . . . . 35
16 Empirical relative bias of posterior estimates for 100-year return levels $Q(.99|\,\boldsymbol{\eta}(\boldsymbol{s}))$ across comparison models and all simulations. . . . . . . . . . . . . . . . . . 36
17 Empirical relative bias of posterior estimates for GEV location parameters $\mu(\boldsymbol{s})$ across comparison models and all simulations . . . . . . . . . . . . . . . . . 37
18 Empirical relative bias of posterior estimates for GEV scale parameters $\sigma(\boldsymbol{s})$ across comparison models and all simulations . . . . . . . . . . . . . . . . . . 38

19 Empirical relative bias of posterior estimates for GEV shape parameters $\xi(\boldsymbol{s})$ across comparison models and all simulations . . . . . . . . . . . . . . . . . . . 39
20 Distribution of likelihood weights (5) for Colorado data and simulations with $N = T = 50$. The Colorado weights suggest the data have moderate extremal dependence. . . . . . . . . . . . . . . . . . . . . . . . . . . . . . . . . . . . . 40
21 Comparison of weighted $\hat{Q}_{wtd}(.99|\,\boldsymbol{\eta}(\boldsymbol{s}))$ and unweighted $\hat{Q}(.99|\,\boldsymbol{\eta}(\boldsymbol{s}))$ return level estimates plotted against a dotted 1:1 reference line. The weighted model shrinks estimates toward a common return level. Shrinkage occurs as unweighted return level estimates below the unweighted average $\bar{Q}$ tend to increase in the weighted model, while unweighted return level estimates above $\bar{Q}$ tend to decrease. . . . . . . . . . . . . . . . . . . . . . . . . . . . . . 41

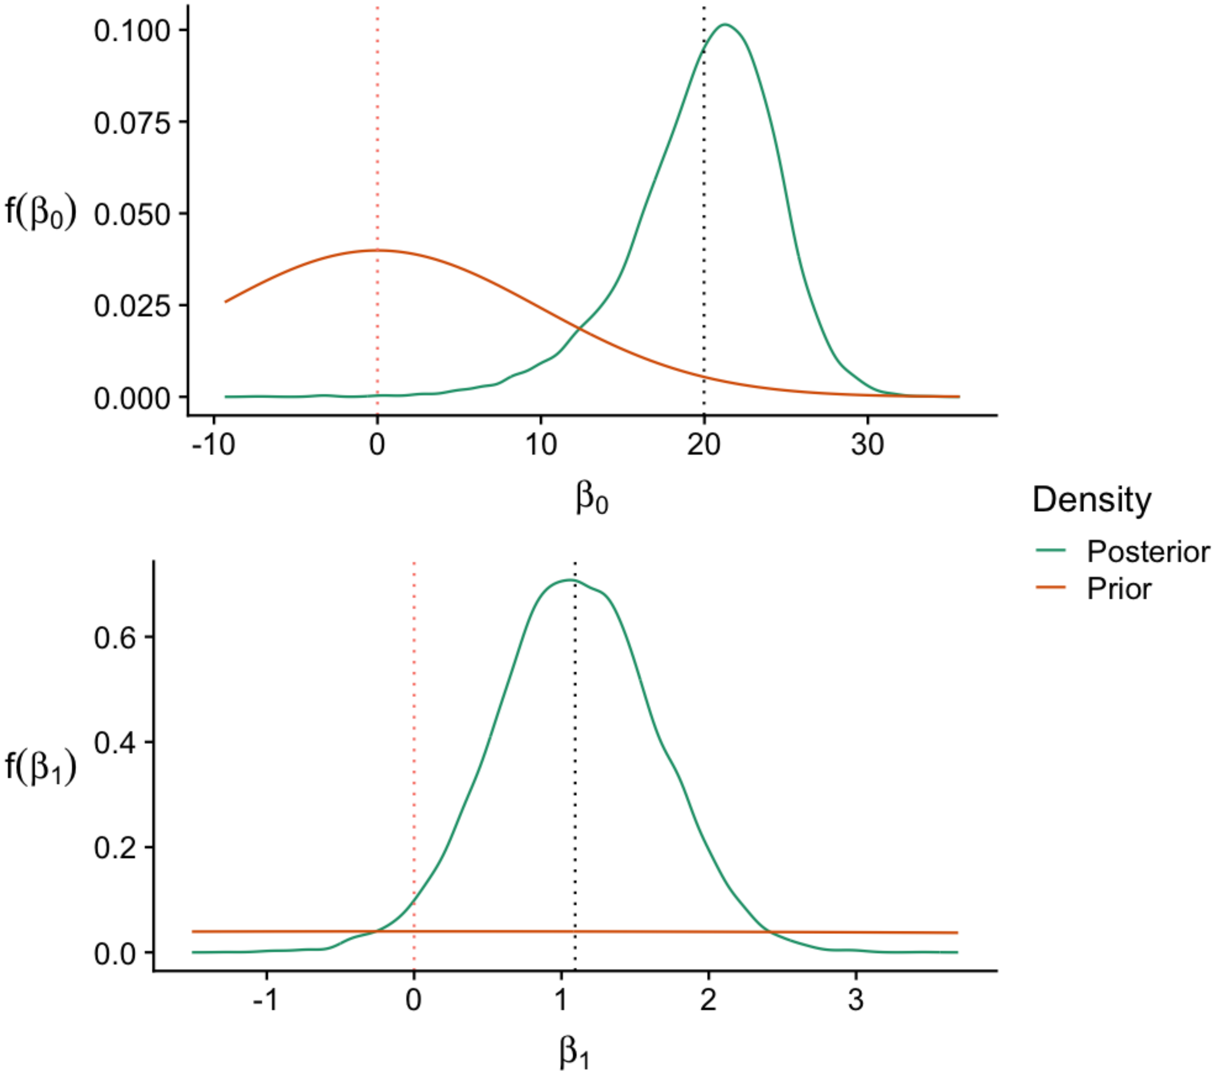


Figure 1: Comparison of prior and posterior distributions for the mean function of the latent Gaussian process that models GEV location parameters $\{\mu(\boldsymbol{s})\}_{\boldsymbol{s}\in\mathcal{D}}$. Prior and posterior means are marked by vertical dotted lines. The plots show strong posterior learning in both the intercept $\beta_0$ and slope parameters $\beta_1$, which model a linear trend between annual average precipitation and GEV location parameters.

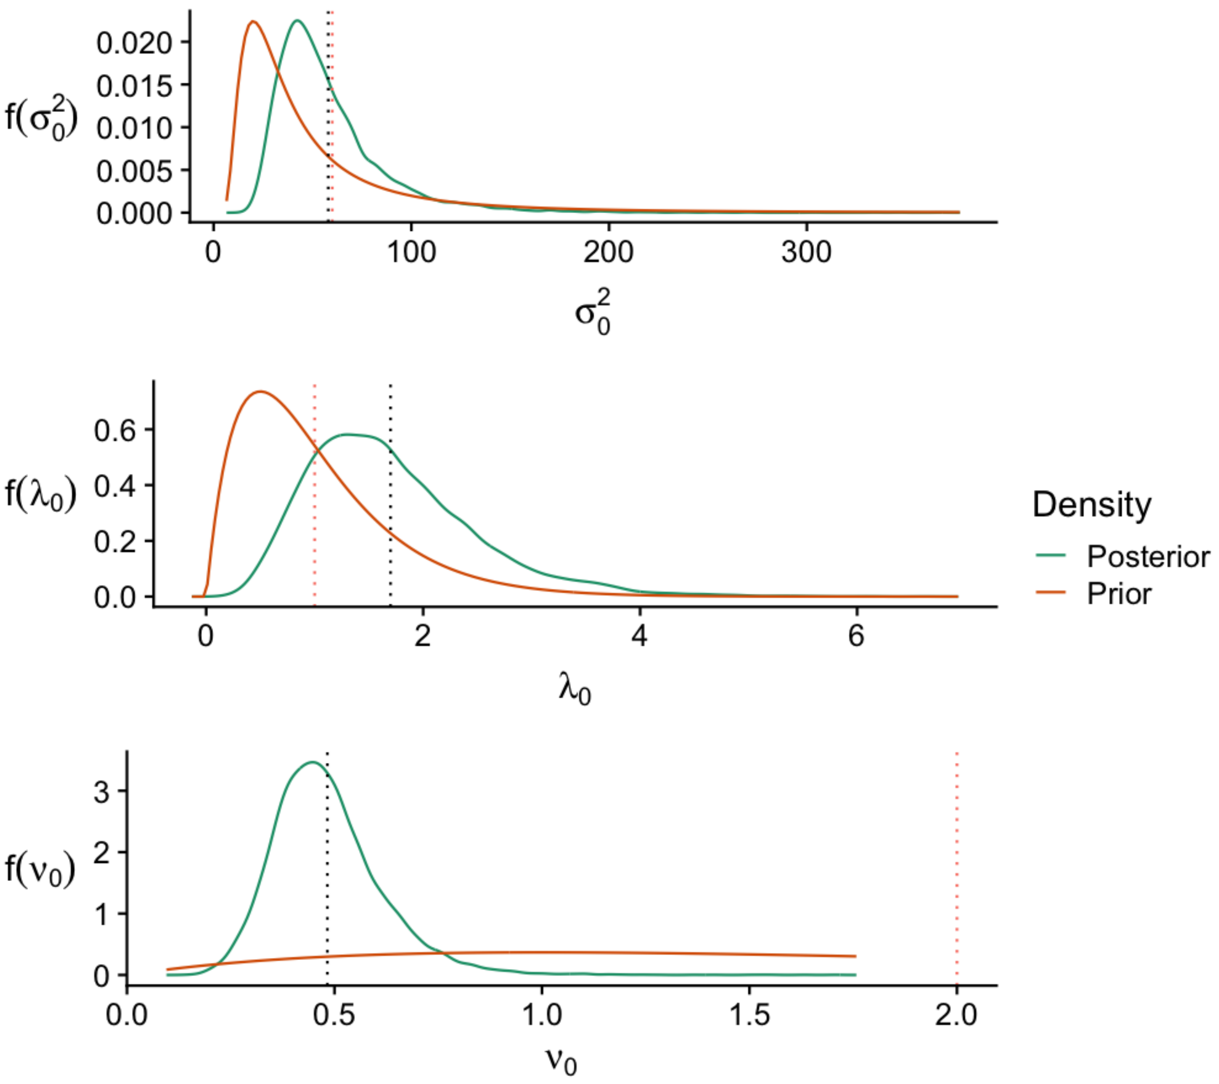


Figure 2: Comparison of prior and posterior distributions for the covariance parameters of the latent Gaussian process that models GEV location parameters $\{\mu(\boldsymbol{s})\}_{\boldsymbol{s}\in\mathcal{D}}$. Prior and posterior means are marked by vertical dotted lines. The plots show strong posterior learning in the covariance range $\lambda_0$ and smoothness $\nu_0$. There is weaker posterior learning in the covariance sill $\sigma_0^2$ parameter.

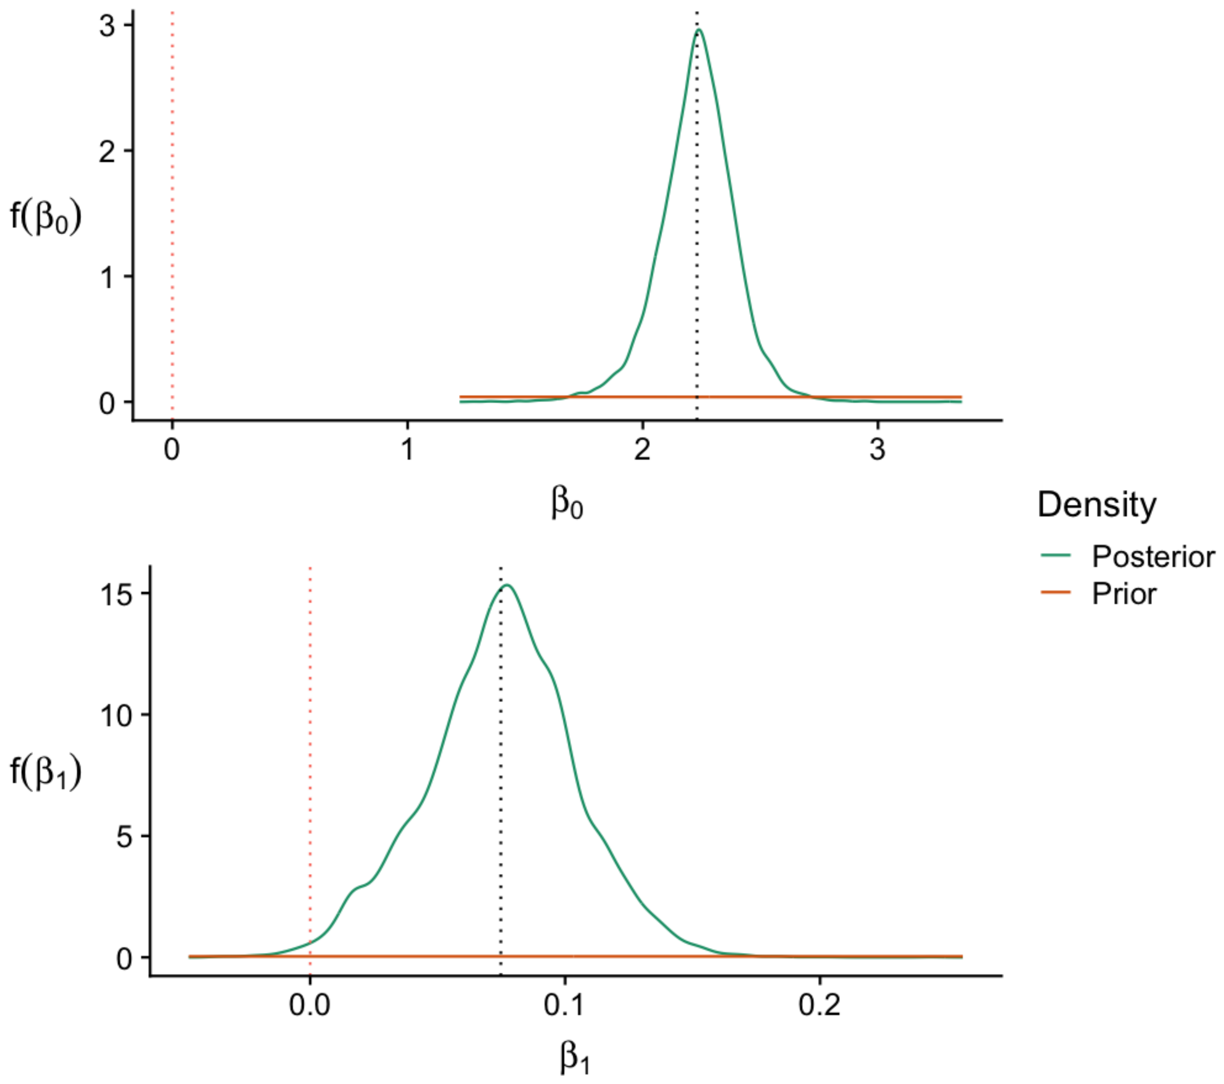


Figure 3: Comparison of prior and posterior distributions for the mean function of the latent Gaussian process that models GEV scale parameters $\{\sigma^2(\boldsymbol{s})\}_{\boldsymbol{s}\in\mathcal{D}}$. Prior and posterior means are marked by vertical dotted lines. The plots show strong posterior learning in both the intercept $\beta_0$ and slope parameters $\beta_1$, which model a linear trend between annual average precipitation and GEV scale parameters.

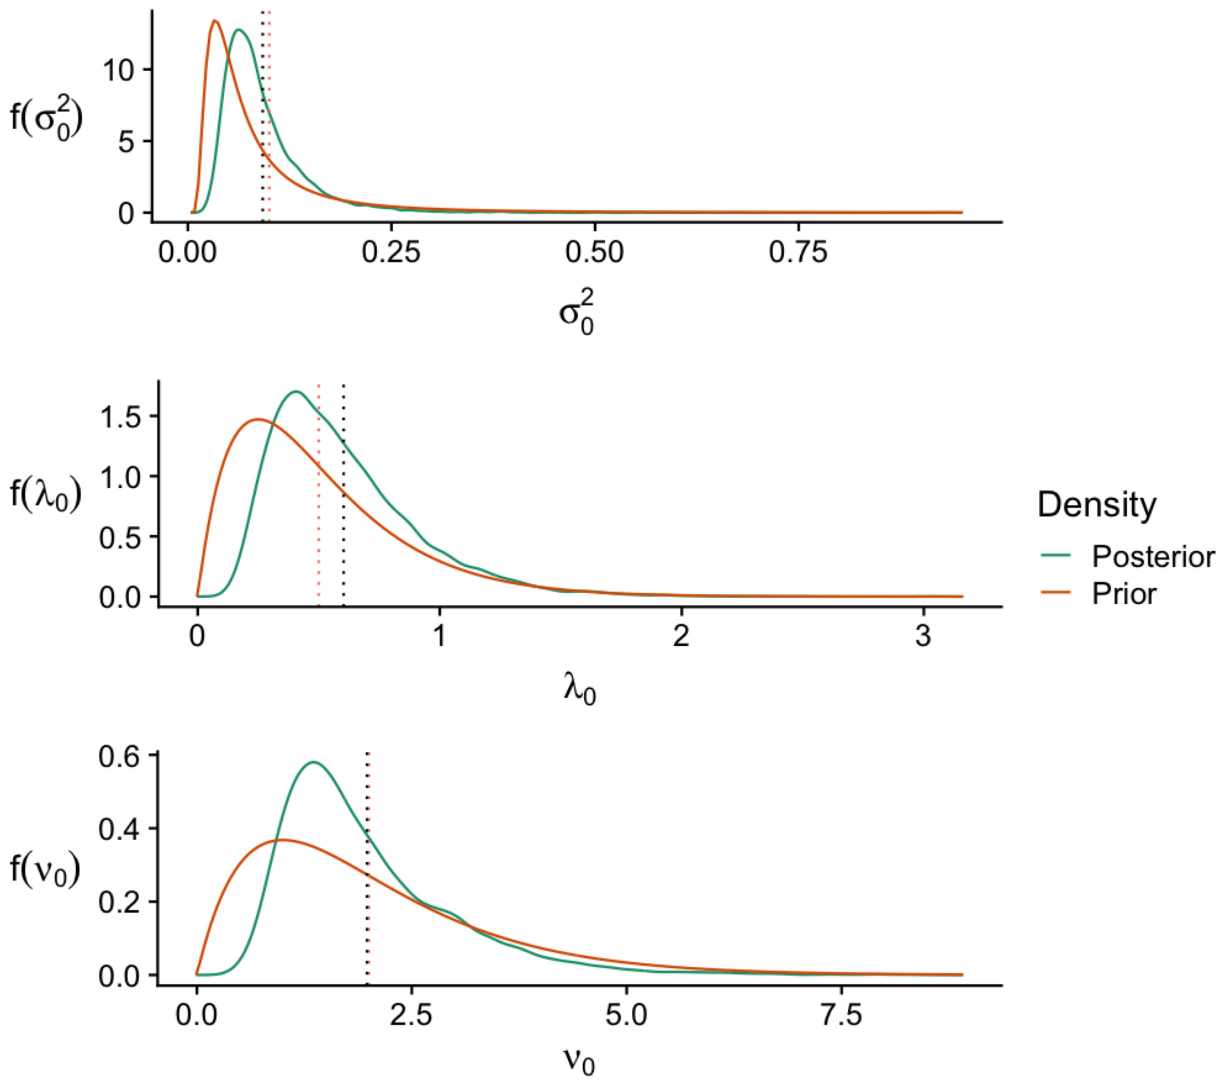


Figure 4: Comparison of prior and posterior distributions for the covariance parameters of the latent Gaussian process that models GEV scale parameters $\{\sigma^2(\boldsymbol{s})\}_{\boldsymbol{s}\in\mathcal{D}}$. Prior and posterior means are marked by vertical dotted lines. The plots show moderate posterior learning in the covariange smoothness $\nu_0$ parameter, but weak posterior learning in the covariance sill $\sigma_0^2$ and range $\lambda_0$ parameters.

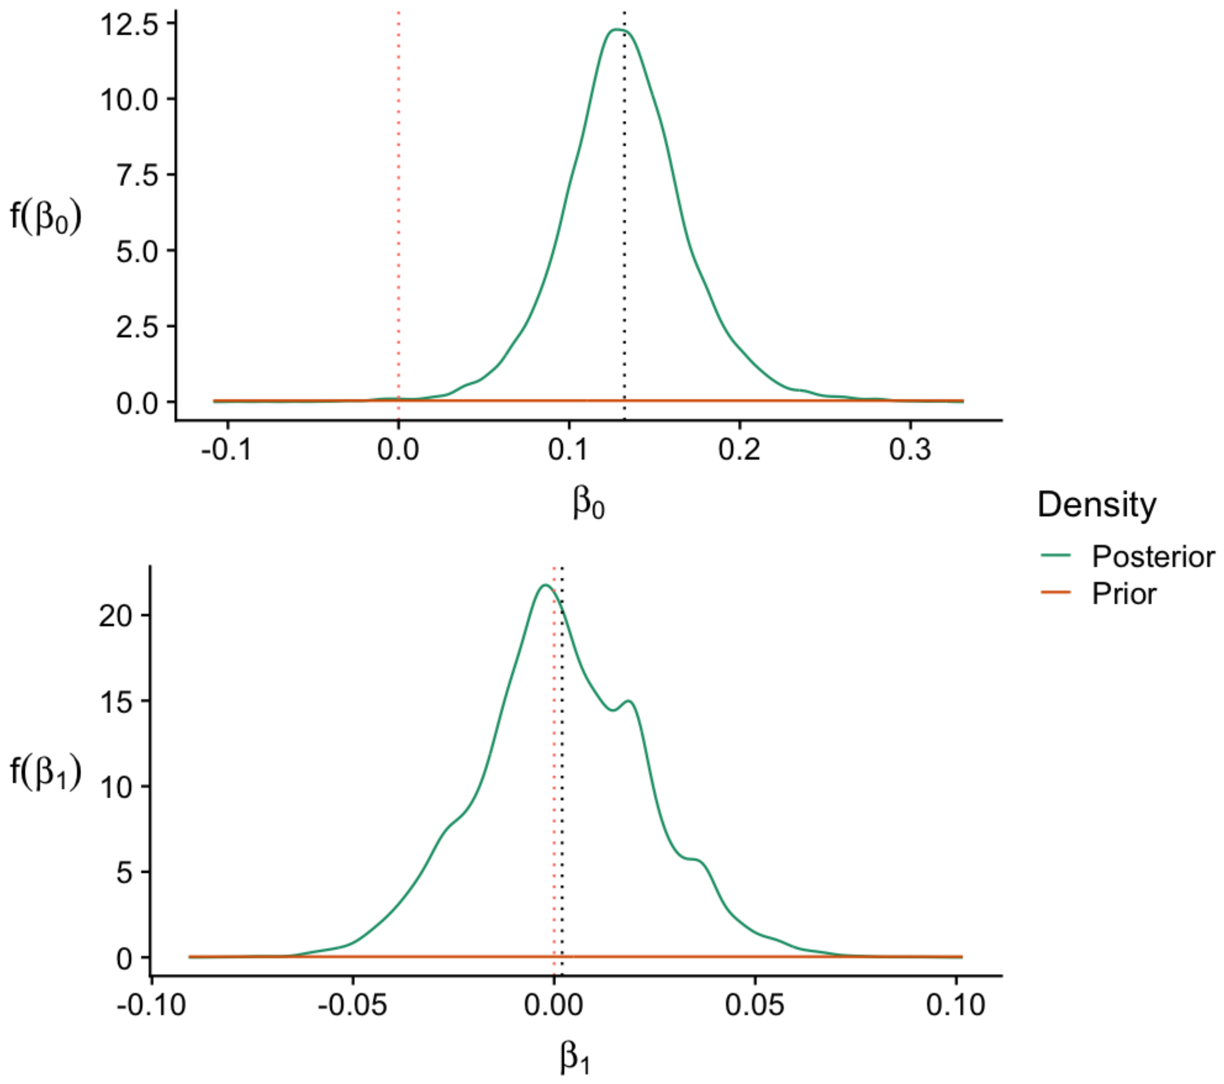


Figure 5: Comparison of prior and posterior distributions for the mean function of the latent Gaussian process that models GEV shape parameters $\{\xi(\boldsymbol{s})\}_{\boldsymbol{s}\in\mathcal{D}}$. Prior and posterior means are marked by vertical dotted lines. The plots show strong posterior learning in both the intercept $\beta_0$ and slope parameters $\beta_1$, which model a deterministic trend between annual average precipitation and GEV shape parameters.

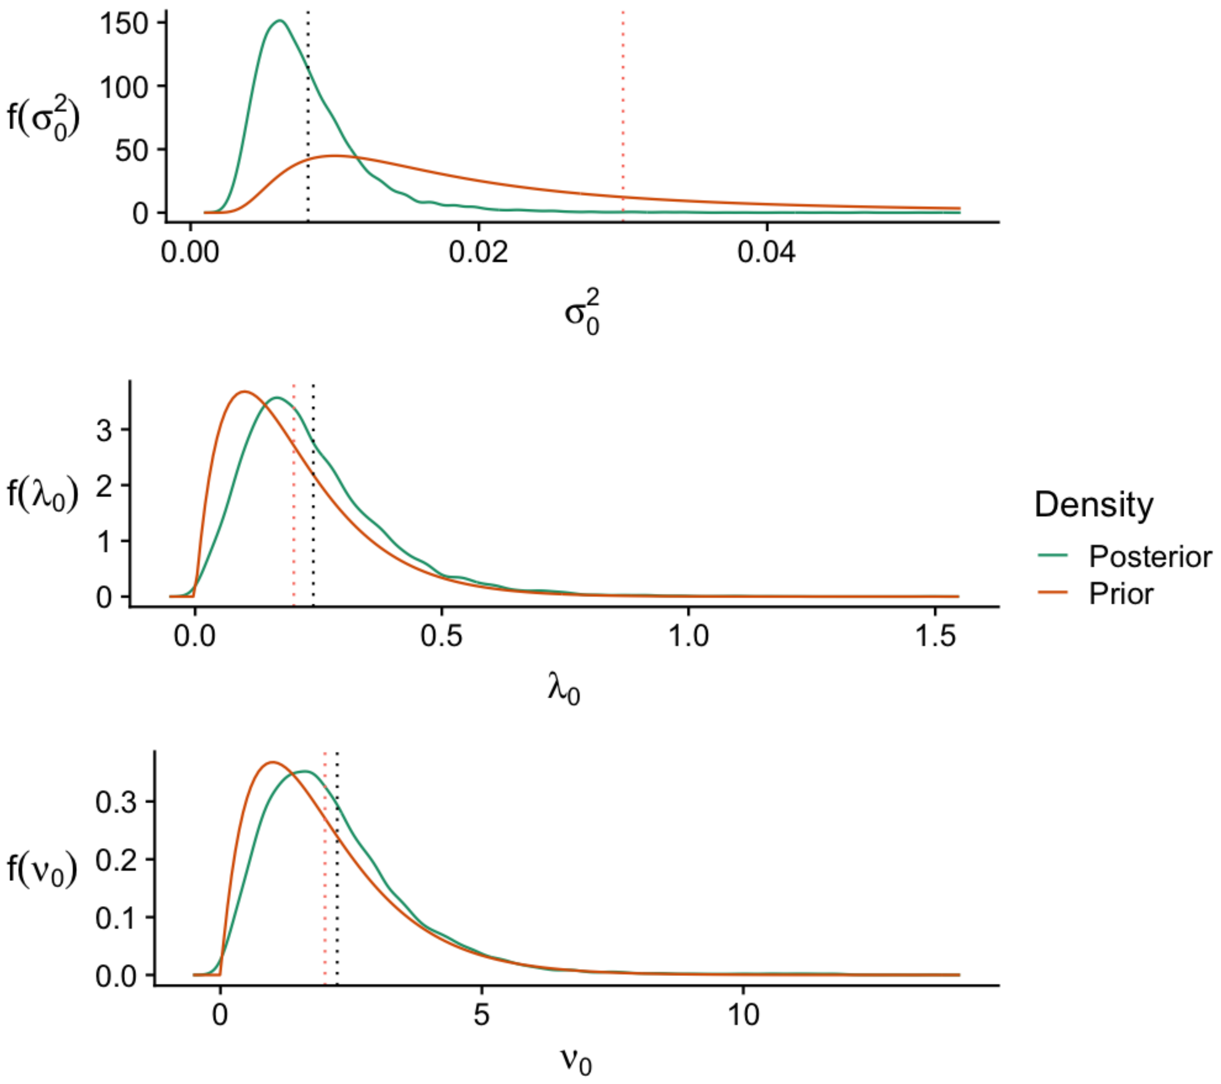


Figure 6: Comparison of prior and posterior distributions for the covariance parameters of the latent Gaussian process that models GEV shape parameters $\{\xi(\boldsymbol{s})\}_{\boldsymbol{s}\in\mathcal{D}}$. Prior and posterior means are marked by vertical dotted lines. The plots show strong posterior learning in the covariance sill $\sigma_0^2$, but almost no posterior learning in the covariance range $\lambda_0$ or smoothness $\lambda_0$ parameters.

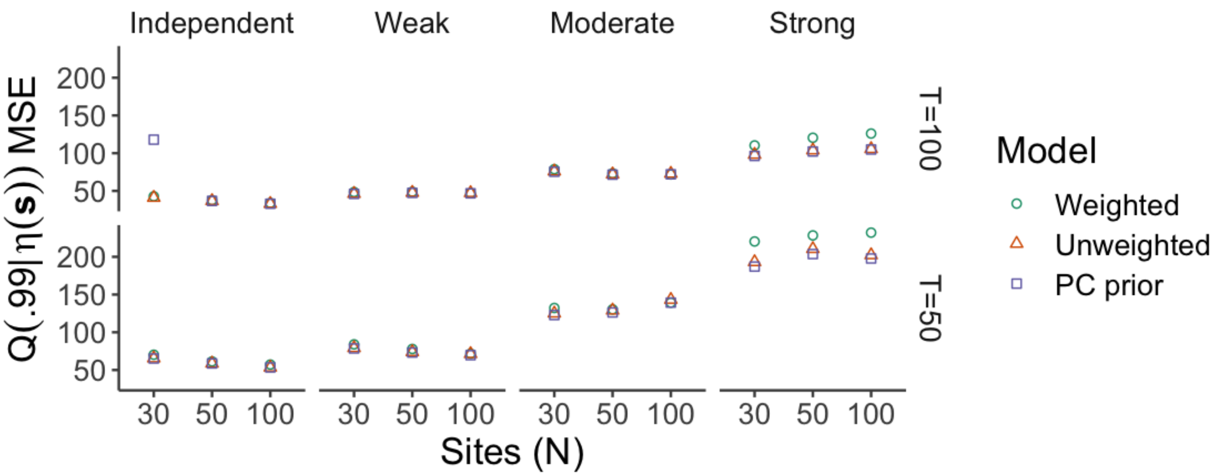


Figure 7: Empirical mean squared error (MSE) of posterior estimates for 100-year return levels $Q(.99|\boldsymbol{\eta}(\boldsymbol{s}))$ for four levels of extreme dependence across comparison models and simulations with $T = 50$ observations per location. The weighted model has similar or better performance than the standard, unweighted model in nearly all simulations. The unweighted model underestimates uncertainty, so has slightly smaller MSE for the simulation with strong extremal dependence. Supplement Section D includes results for $T = 100$, which show slight reduction in MSE.

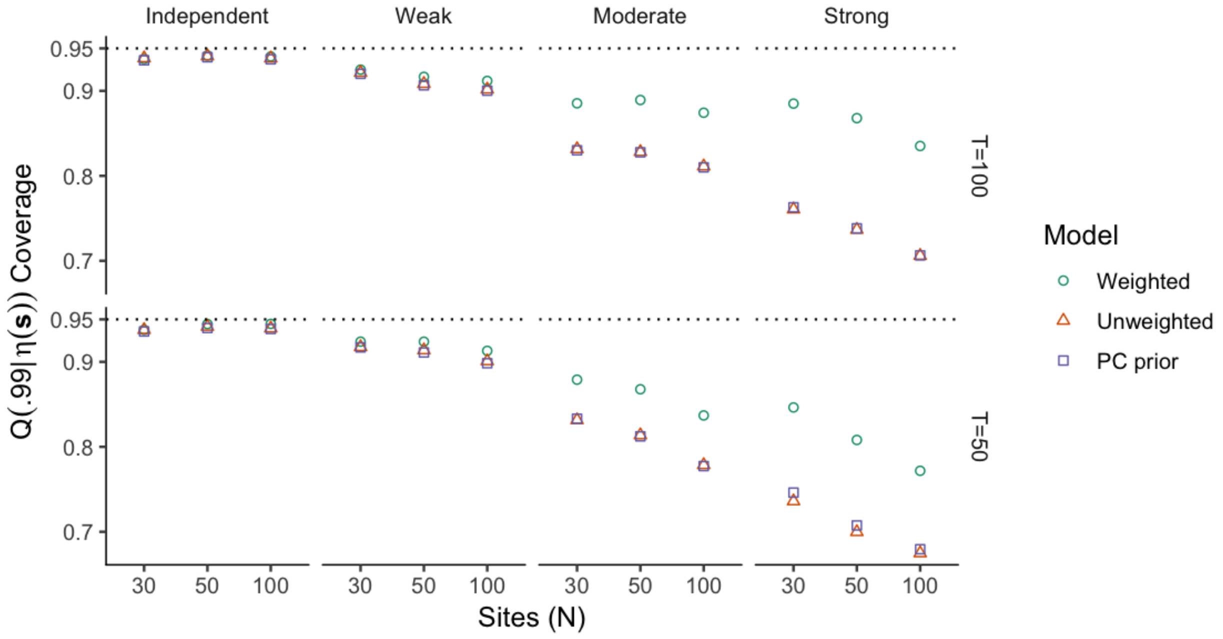


Figure 8: Empirical coverage rates of 95% highest posterior density intervals for 100-year return levels $Q(.99|\,\boldsymbol{\eta}(\boldsymbol{s}))$ across comparison models and all simulations. Nominal coverage is marked by the dotted horizontal reference line at .95.

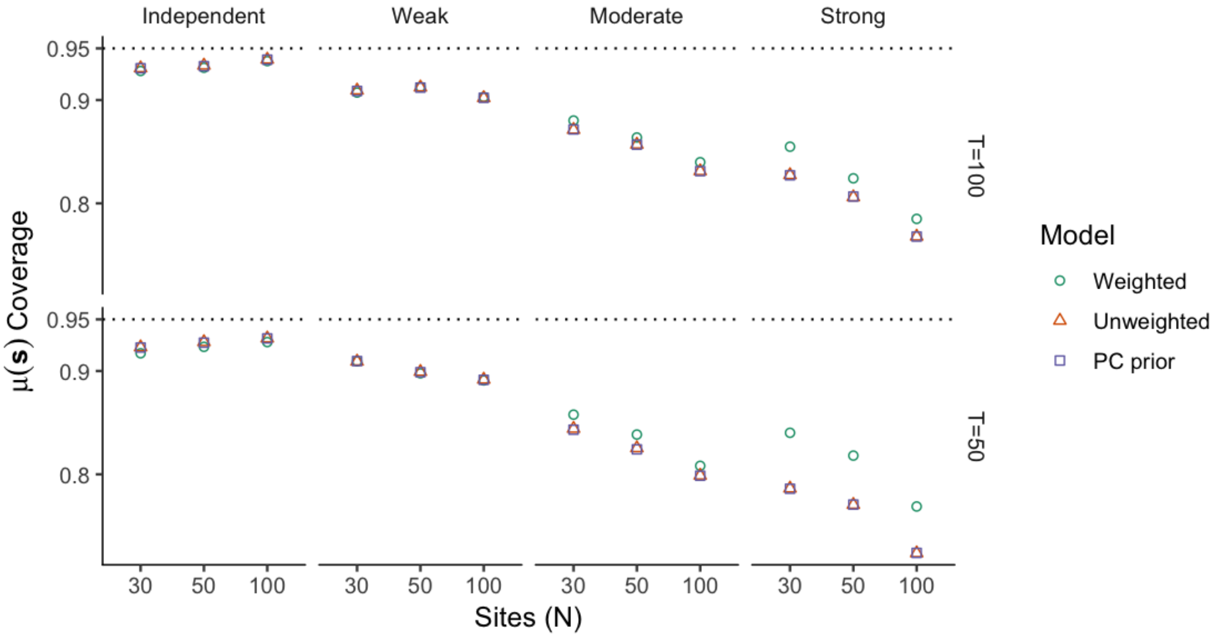


Figure 9: Empirical coverage rates of 95% highest posterior density intervals for GEV location parameters $\mu(\boldsymbol{s})$ across comparison models and all simulations. Nominal coverage is marked by the dotted horizontal reference line at .95.

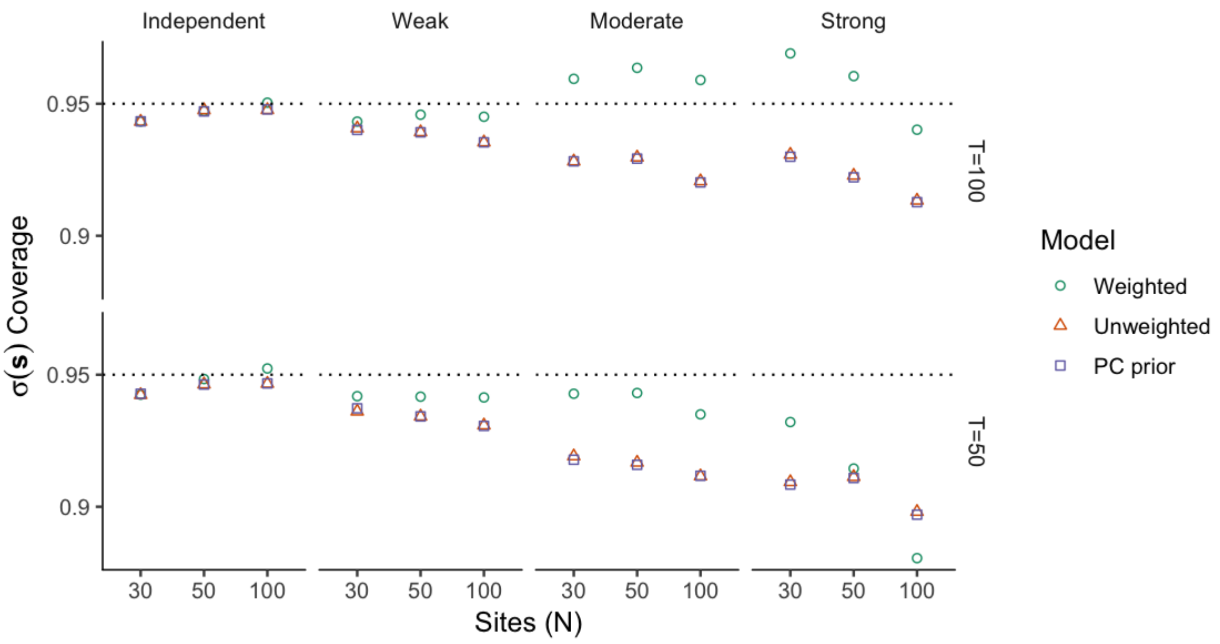


Figure 10: Empirical coverage rates of 95% highest posterior density intervals for GEV scale parameters $\sigma(\boldsymbol{s})$ across comparison models and all simulations. Nominal coverage is marked by the dotted horizontal reference line at .95.

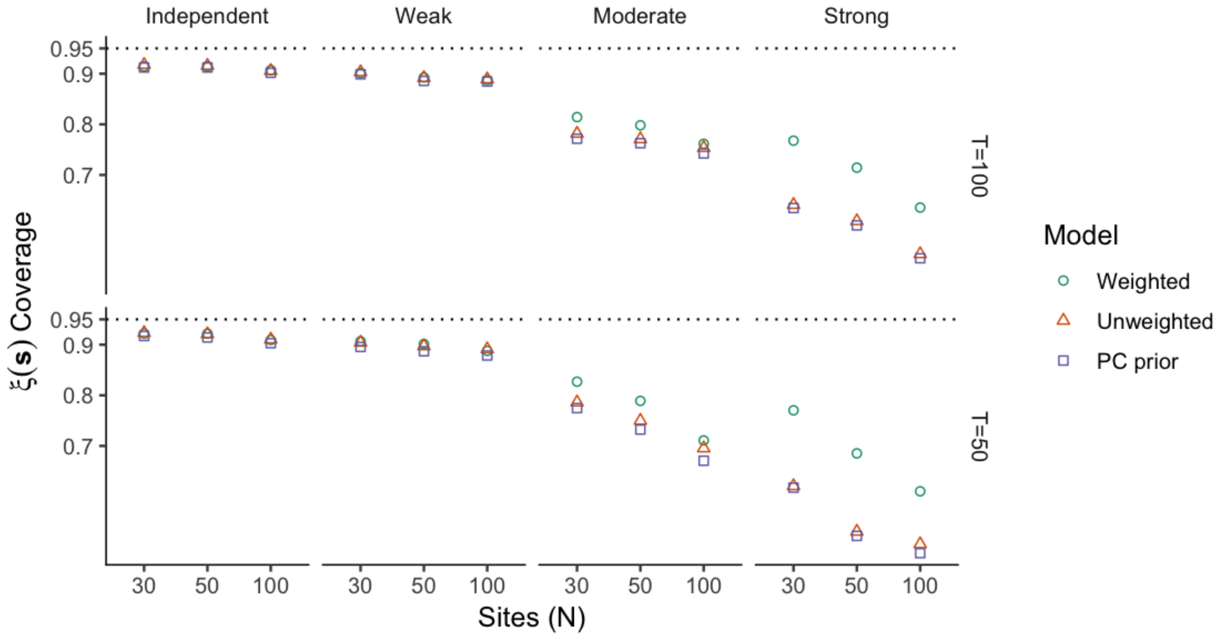


Figure 11: Empirical coverage rates of 95% highest posterior density intervals for GEV shape parameters $\xi(\boldsymbol{s})$ across comparison models and all simulations. Nominal coverage is marked by the dotted horizontal reference line at .95.

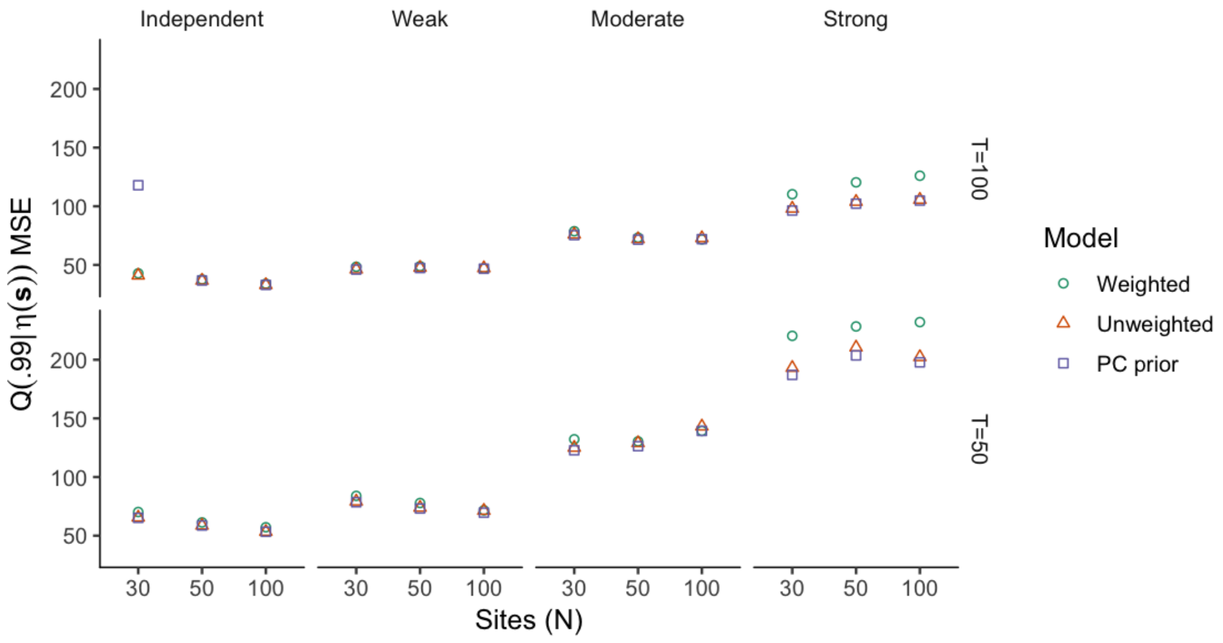


Figure 12: Empirical mean square error (MSE) of posterior estimates for 100-year return levels $Q(.99|\,\boldsymbol{\eta}(\boldsymbol{s}))$ across comparison models and all simulations.

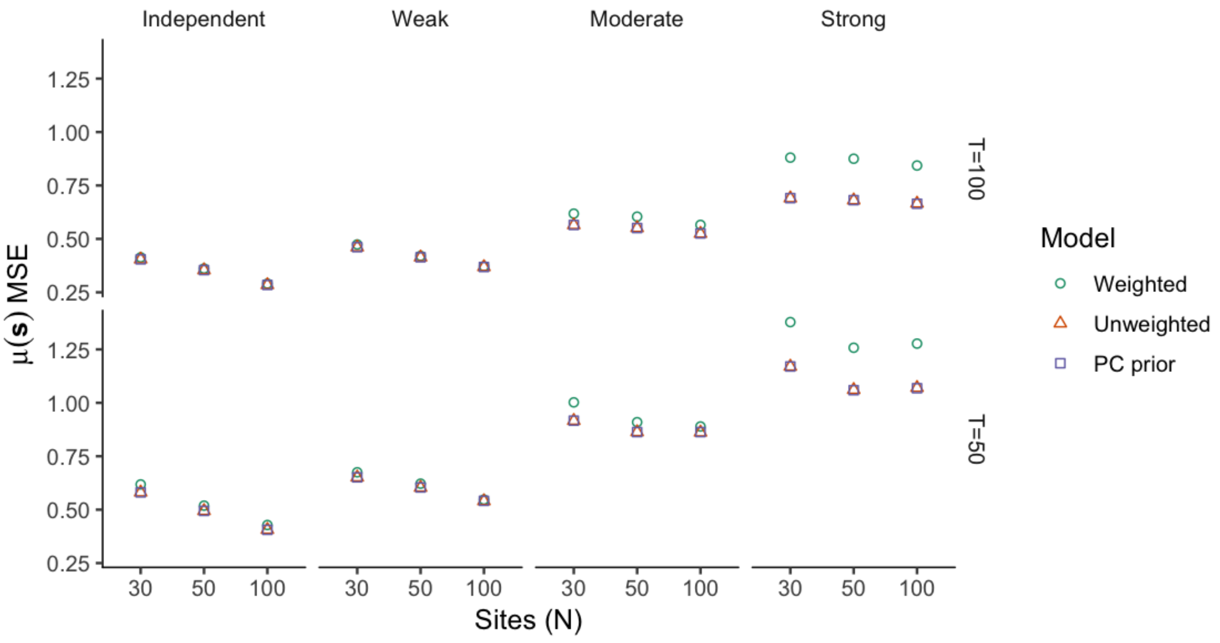


Figure 13: Empirical mean square error (MSE) of posterior estimates for GEV location parameters $\mu(\boldsymbol{s})$ across comparison models and all simulations.

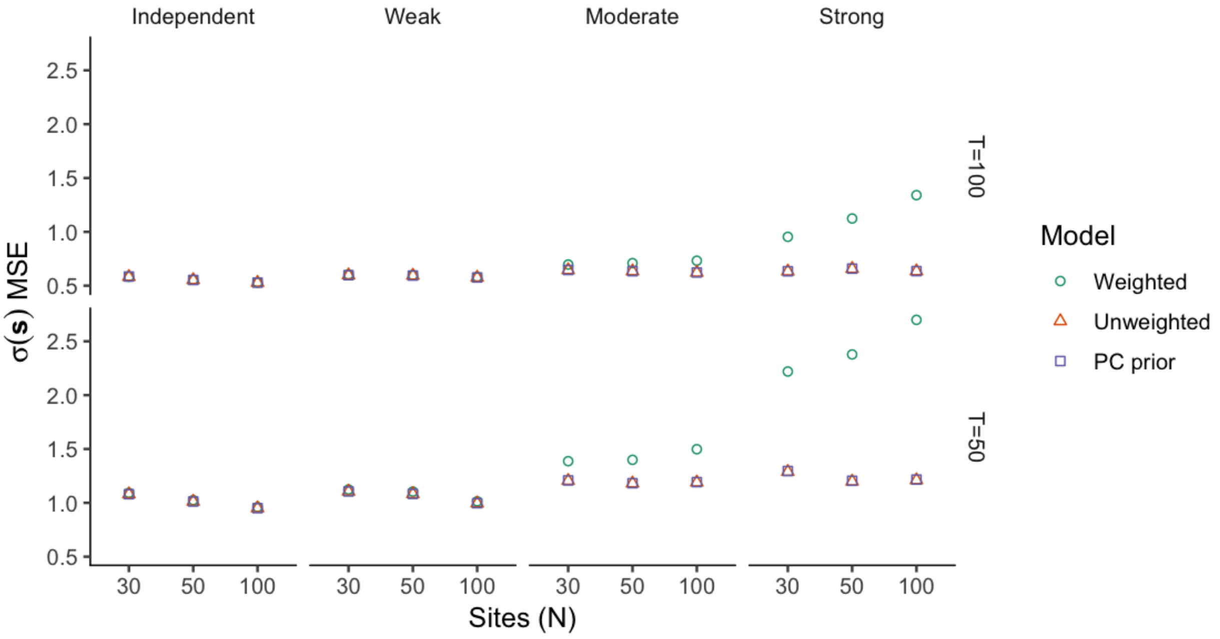


Figure 14: Empirical mean square error (MSE) of posterior estimates for GEV scale parameters $\sigma(\boldsymbol{s})$ across comparison models and all simulations.

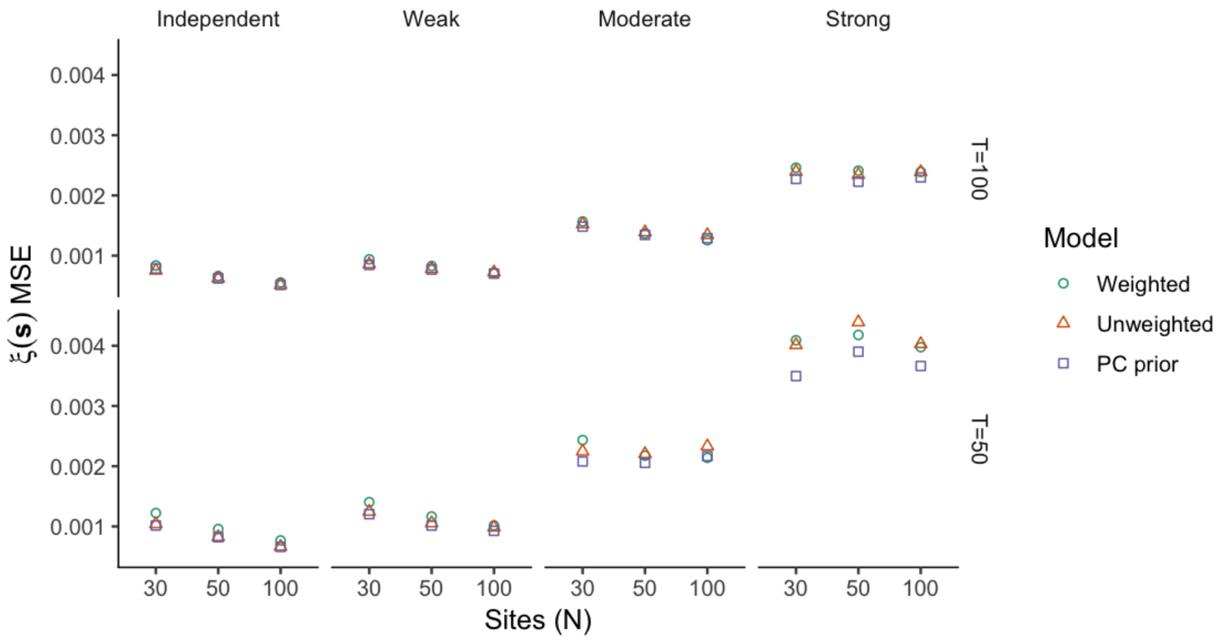


Figure 15: Empirical mean square error (MSE) of posterior estimates for GEV shape parameters $\xi(\boldsymbol{s})$ across comparison models and all simulations.

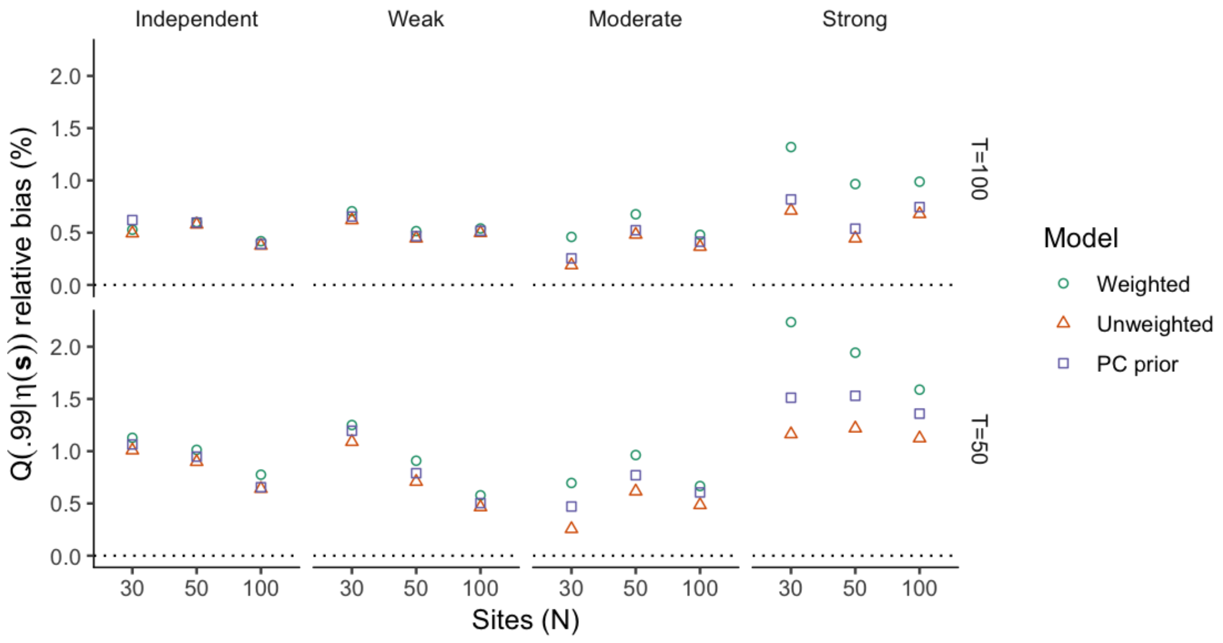


Figure 16: Empirical relative bias of posterior estimates for 100-year return levels $Q(.99|\,\boldsymbol{\eta}(\boldsymbol{s}))$ across comparison models and all simulations.

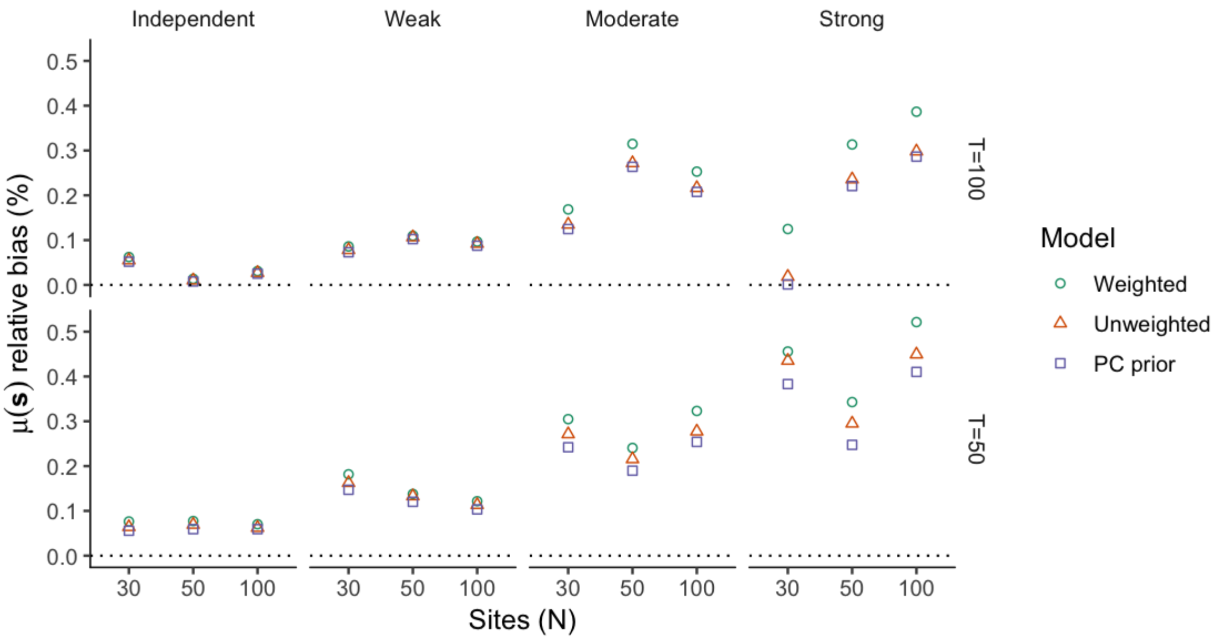


Figure 17: Empirical relative bias of posterior estimates for GEV location parameters $\mu(\boldsymbol{s})$ across comparison models and all simulations.

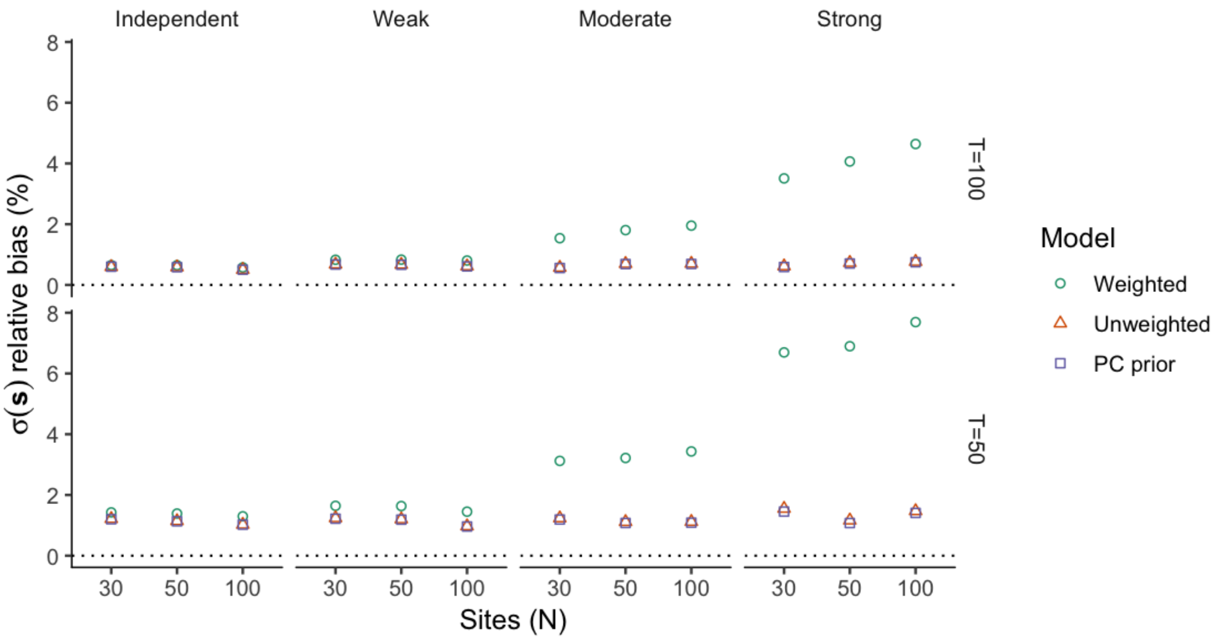


Figure 18: Empirical relative bias of posterior estimates for GEV scale parameters $\sigma(\boldsymbol{s})$ across comparison models and all simulations.

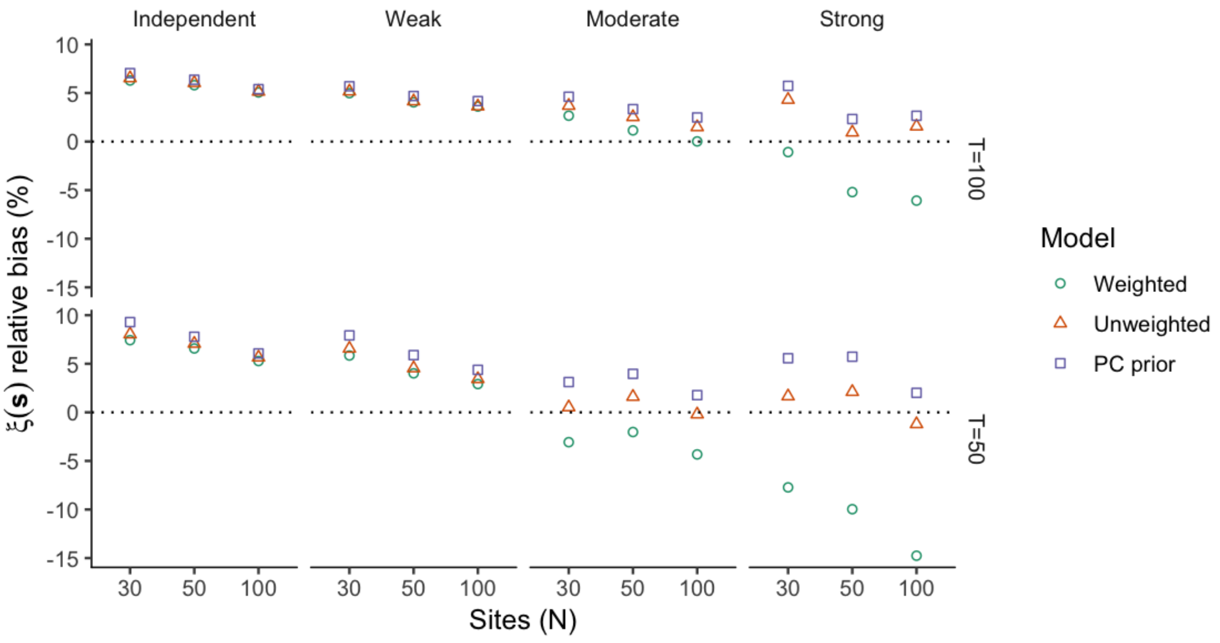


Figure 19: Empirical relative bias of posterior estimates for GEV shape parameters $\xi(\boldsymbol{s})$ across comparison models and all simulations.

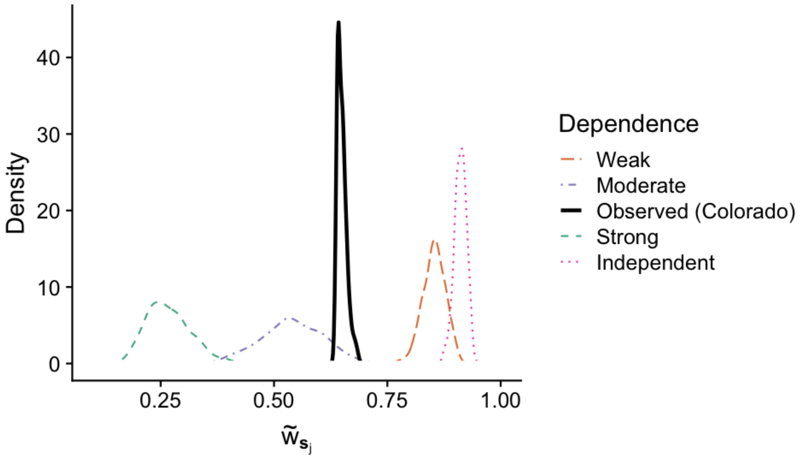


Figure 20: Distribution of likelihood weights (5) for Colorado data and simulations with $N = T = 50$. The Colorado weights suggest the data have moderate extremal dependence.

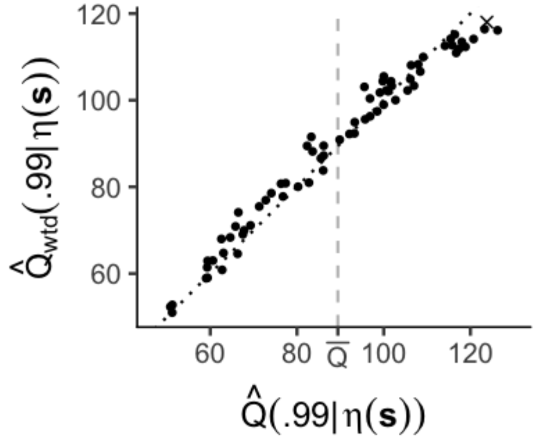


Figure 21: Comparison of weighted $\hat{Q}_{wtd}(.99|\,\boldsymbol{\eta}(\boldsymbol{s}))$ and unweighted $\hat{Q}(.99|\,\boldsymbol{\eta}(\boldsymbol{s}))$ return level estimates plotted against a dotted 1:1 reference line. The weighted model shrinks estimates toward a common return level. Shrinkage occurs as unweighted return level estimates below the unweighted average $\bar{Q}$ tend to increase in the weighted model, while unweighted return level estimates above $\bar{Q}$ tend to decrease.
